# Supplementary material for: Robust Ranking Explanations
Source: arXiv:2307.04024 source file (2023-07-08)
Supplement: Supplementary file 1 [file supp.tex]

\clearpage
\newpage
\appendix

\section{Proofs}
% Start from pairwise ranking thickness, e.g., 
% % Eq. (\ref{eq:pairwise_rank_thick}).
% maximize $\int_0^1 h(\mathbf{x}(t),i,j) dt$.
\subsection{Bounds of Ranking Explanation Thickness}
\label{sec:appendix-proof-bounds}
In this section,
we explore the lower and upper bounds of the \textit{relaxed} ranking explanation thickness without indicator function.
We denote $\mathbf{x}$ as the target sample,
$\|\delta\|_2 \leq \epsilon$ as the perturbation, 
$\mathbf{x}^\prime=\mathbf{x}+\delta$ as the perturbed input,
and $\mathbf{x}(t)=(1-t)\mathbf{x} + t \mathbf{x}^\prime, t \in [0,1]$.
% as indicated in Eq. (\ref{eq:attack_general}).

\begin{proposition}
% \begin{theorem}
[Bounds of Local Ranking Explanation Thickness]
Given a $L$-locally Lipschitz model $f(\mathbf{x})$,
for some 
% $L$ that
% (
$L \geq \frac{ \|\mathbf{x}-\mathbf{x}^\ast\|_2 * \max_i 
% \max_{\mathbf{x}^\prime\in B_2(\mathbf{x},\epsilon)} \|H(\mathbf{x}^\prime)_i\|_2}
L_i}
{2}$ 
where 
$\mathbf{x}^\ast = \argmax_{\mathbf{x}^\prime \in \mathcal{B}_2(\mathbf{x},\epsilon)}\frac{\|\mathcal{I}(\mathbf{x}) - \mathcal{I}(\mathbf{x}^\prime)\|_2}{\|\mathbf{x}-\mathbf{x}^\prime\|}$,
% \textit{[Plan to put it in the appendix]}
% )
% then
the \textit{relaxed} local ranking explanation thickness for ($i,j$) pair of a target $\mathbf{x}$ is bounded by 
\begin{equation*}
\begin{aligned}
    % g(\mathbf{x}_r)_i - g(\mathbf{x}_r)_j -
    & h(\mathbf{x},i,j) - 
    \epsilon * \frac{1}{2} \|H(\mathbf{x})_i -H(\mathbf{x})_j\|_2
    \leq \\
    & \mathbb{E}_{\mathbf{x}^\prime} 
    \left[ \int_0^1 h(\mathbf{x}(t),i,j) dt
    \right]
    \leq
    % g(\mathbf{x}_r)_i - g(\mathbf{x}_r)_j +
    h(\mathbf{x},i,j) +
    \epsilon * (L_i + L_j),
\end{aligned}
\end{equation*}
where $H(\mathbf{x})_i$ is the $i$-th column of Hessian matrix of $f$ with respect to the input $\mathbf{x}$,
and 
$L_i=\max_{\mathbf{x}^\prime \in \mathcal{B}_2(\mathbf{x},\epsilon)} \| H(\mathbf{x}^\prime)_i \|_2$.
\end{proposition}
% \end{theorem}

\noindent \textbf{Lower bound.}
% First, 
% we try to find the lower bound for the ranking thickness of a target sample $\mathbf{x}_r$.
% Denote 
% $\|\delta\|_2 \leq \epsilon$ as the perturbation, 
% $\mathbf{x}_s=\mathbf{x}_r+\delta$ as the perturbed input,
% and $\mathbf{x}(t)=(1-t)\mathbf{x}_r + t \mathbf{x}_s, t \in [0,1]$
% as indicated in Eq. (\ref{eq:attack_general}).
We start from the definition of local ranking thickness between ($i,j$) pair of explanations of $\mathbf{x}$ in Eq. (\ref{eq:pairwise_rank_thick}) without indicator function.
\begin{equation}
\label{eq:thickness_lower_bound}
\begin{aligned}
    % \max_f 
    & 
    % \mathbb{E}_{(\mathbf{x}_r,\mathbf{x}_s)\sim \mathcal{D}}
    \int_0^1 h(\mathbf{x}(t), i,j) dt 
    \\ = &
    \int_0^1 \mathcal{I}(\mathbf{x}(t))_i - \mathcal{I}(\mathbf{x}(t))_j dt
    \\ = &
    \int_0^1 \mathcal{I}(\mathbf{x} + t\delta)_i - \mathcal{I}(\mathbf{x} + t\delta)_j dt
    \\ \approx &
    \int_0^1 \mathcal{I}(\mathbf{x})_i + t\delta^\top H(\mathbf{x})_i -
    \mathcal{I}(\mathbf{x})_j - t\delta^\top H(\mathbf{x})_j dt
    \\ = &
    \mathcal{I}(\mathbf{x})_i - \mathcal{I}(\mathbf{x})_j + 
    \frac{\delta^\top}{2} H(\mathbf{x})_i -
    \frac{\delta^\top}{2} H(\mathbf{x})_j
    \\ \geq &
    \mathcal{I}(\mathbf{x})_i - \mathcal{I}(\mathbf{x})_j - 
    \epsilon * \frac{1}{2} \|H(\mathbf{x})_i -H(\mathbf{x})_j\|_2
    ,
\end{aligned}
\end{equation}
% where $H(\mathbf{x})_i$ is the $i$-th column of Hessian matrix of $f$ with respect to $\mathbf{x}$.
% Line-2 holds due to the definition of $h(\mathbf{x},i,j)=g(\mathbf{x})_i - g(\mathbf{x})_j$.
On line-4, 
we apply the Taylor Expansion to
% obtain the approximation of 
approximate the gradient at intermediate point $\mathbf{x}+t\delta$.
Then we find the minimum 
with
% by setting 
$\delta = 
\argmin_{ \|\delta\|\leq \epsilon} 
\frac{1}{2} \delta^\top(H(\mathbf{x})_i - H(\mathbf{x})_j)
= -\epsilon \frac{H(\mathbf{x})_i-H(\mathbf{x})_j}{\|H(\mathbf{x})_i-H(\mathbf{x})_j\|_2}$ on line-6.

% [Note that $H(\mathbf{x}_r)_i= H(\mathbf{x}_r)_j, \forall i\in \{1,\dots,k\},j\in\{ k+1,\dots,n \}$ results in $H(\mathbf{x}_r)_i= H(\mathbf{x}_r)_j, \forall i,j\in \{1,\dots,n\}$,
% which makes the determinant of $H$ be zero
% due to the symmetry of Hessian matrix $H$.]

\noindent \textbf{Upper bound.}
% We provide the proofs for the upper bound.
Before the proofs for the upper bound,
we introduce the lemmas from \cite{paulavivcius2006analysis} and \cite{wang2020smoothed}.
% respectively.
\begin{lemma}
\label{lemma:gradient_lipschitz}
If a function $g:\mathbb{R}^n\to \mathbb{R}$ is $L$-locally Lipschitz within $\mathcal{B}_p(\mathbf{x},\epsilon)$,
such that 
$ |g(\mathbf{x}) - g(\mathbf{x}^\prime) | \leq L \| \mathbf{x} - \mathbf{x}^\prime \|_p, \;  \forall \mathbf{x}^\prime \in \mathcal{B}_p(\mathbf{x},\epsilon) = \{ \mathbf{x}^\prime  : \| \mathbf{x}^\prime - \mathbf{x} \|_p \leq \epsilon \}$, 
then
\begin{equation}
    L = \max_{\mathbf{x}^\prime\in \mathcal{B}_p(\mathbf{x},\epsilon)} \| \nabla_{\mathbf{x}^\prime} g(\mathbf{x}^\prime) \|_q,
\end{equation}
where $\frac{1}{p}+\frac{1}{q}=1,1\leq p,q\leq \infty$.
\end{lemma}

\begin{lemma}
\label{lemma:lipschitz_chain_rule}
If a function $f(\mathbf{x})$ is $L$-locally Lipschitz continuous in $\mathcal{B}_2(\mathbf{x},\epsilon)$,
then $\mathcal{I}(\mathbf{x})$ is $K$-locally Lipschitz as well,
where $K \leq \frac{2L}{\|\mathbf{x}-\mathbf{x}^\ast \|}$
and $\mathbf{x}^\ast = \argmax_{\mathbf{x}^\prime \in \mathcal{B}_2(\mathbf{x},\epsilon)} \frac{\|\mathcal{I}(\mathbf{x}) - \mathcal{I}(\mathbf{x}^\prime) \|_2}{\| \mathbf{x} - \mathbf{x}^\prime \|_2}$.
\end{lemma}

We now start our proofs from $L$-locally Lipschitz $f(\mathbf{x})$.
% with $L \geq \frac{ \|\mathbf{x}-\mathbf{x}^\ast\|_2 * \max_i L_i}{2}$.
Based on Lemma \ref{lemma:lipschitz_chain_rule},
we know that $\mathcal{I}(\mathbf{x})$ is $K$-locally Lipschitz,
where $K \leq \frac{2L}{\|\mathbf{x}-\mathbf{x}^\ast\|}$.
Based on Definition \ref{definition:locally_lipschitz},
it is safe to claim that 
$\forall i, 
\mathcal{I}(\mathbf{x})_i : \mathbb{R}^n \to \mathbb{R}$,
any entry of $\mathcal{I}(\mathbf{x})$,
is $K$-locally Lipschitz as well.
\begin{equation*}
    | \mathcal{I}(\mathbf{x})_i - \mathcal{I}(\mathbf{x}^\prime)_i |
    \leq
    \| \mathcal{I}(\mathbf{x}) - \mathcal{I}(\mathbf{x}^\prime) \|_2
    \leq
    K \| \mathbf{x} - \mathbf{x}^\prime \|_2.
\end{equation*}
Specifically,
we denote the locally Lipschitz constant for $\mathcal{I}(\mathbf{x})_i$ as $L_i \leq K$,
and based on Lemma \ref{lemma:gradient_lipschitz},
we have 
$L_i 
= \max_{\mathbf{x}^\prime\in \mathcal{B}_2(\mathbf{x},\epsilon)} \| \nabla_{\mathbf{x}^\prime} \mathcal{I}(\mathbf{x}^\prime)_i \|_2 
= \max_{\mathbf{x}^\prime\in \mathcal{B}_2(\mathbf{x},\epsilon)} \|
H(\mathbf{x}^\prime)_i \|_2
$ by taking $p=q=2$.

% Given that $\mathcal{I}(\mathbf{x})_i$, $\forall i$, is $L_i$-locally Lipschitz
% within $B_2(\mathbf{x}, \epsilon)$,
% such that 
% $ |g(\mathbf{x})_i - g(\mathbf{x}^\prime)_i | \leq L \| \mathbf{x} - \mathbf{x}^\prime \|_2, \;  \forall \mathbf{x}^\prime \in B_2(\mathbf{x},\epsilon)$.

\begin{equation}
\label{eq:thickness_upper_bound}
\begin{aligned}
    % \max_f 
    & 
    \int_0^1 h(\mathbf{x}(t), i,j) dt 
    \\ = &
    h(\mathbf{x}^\prime_0,i,j)
    \\ = &
    (\mathcal{I}(\mathbf{x}^\prime_0)_i - \mathcal{I}(\mathbf{x})_i) -
    (\mathcal{I}(\mathbf{x}^\prime_0)_j - \mathcal{I}(\mathbf{x})_j) +
    (\mathcal{I}(\mathbf{x})_i - \mathcal{I}(\mathbf{x})_j)
    \\ \leq &
    | \mathcal{I}(\mathbf{x}^\prime_0)_i - \mathcal{I}(\mathbf{x})_i | +
    | \mathcal{I}(\mathbf{x}^\prime_0)_j - \mathcal{I}(\mathbf{x})_j | +
    (\mathcal{I}(\mathbf{x})_i - \mathcal{I}(\mathbf{x})_j)
    \\ \leq &
    L_i \| \mathbf{x}^\prime_0 - \mathbf{x} \|_2 +
    L_j \| \mathbf{x}^\prime_0 - \mathbf{x} \|_2 +
    (\mathcal{I}(\mathbf{x})_i - \mathcal{I}(\mathbf{x})_j)
    \\ \leq &
    \epsilon * (L_i + L_j) +
    (\mathcal{I}(\mathbf{x})_i - \mathcal{I}(\mathbf{x})_j).
\end{aligned}
\end{equation}
Based on first mean value theorem,
there exists a point $\mathbf{x}^\prime_0$ within the line segment $\mathbf{x}$ and $\mathbf{x}^\prime$ such that $h(\mathbf{x}^\prime_0)=\int_0^1 h(\mathbf{x}(t), i,j) dt$ on line-2.
The inequality on line-4 holds since $\mathcal{I}(\mathbf{x})_i:\mathbb{R}^n\to\mathbb{R}$ is a scalar function,
and any scalar is less than or equivalent to its absolute value.
% and the equality holds when $(g(\mathbf{x}_s^0)_i - g(\mathbf{x}_r)_i)\geq 0$.
The inequality on line-5 holds due to $L_i$-locally Lipschitz of $\mathcal{I}(\mathbf{x})_i$ and Lemma \ref{lemma:gradient_lipschitz} with $p=q=2$.
% Specifcally,
% $L_i=\max_{\mathbf{x}^\prime \in B(\mathbf{x},\delta_2)} \| H(\mathbf{x}^\prime)_i \|_2$
% and similar case for $L_j$.
The inequality on line-6 holds due to the fact that $\mathbf{x}^\prime_0$ locates within $\mathcal{B}_2(\mathbf{x}, \epsilon)$.

Now we find the specific $L$ for the upper bound.
Notice that $K\leq\frac{2L}{\| \mathbf{x} - \mathbf{x}^\ast \|}$ and 
$L_i = \max_{\mathbf{x}^\prime\in \mathcal{B}_2(\mathbf{x},\epsilon)} \| H(\mathbf{x}^\prime)_i \|_2 \leq K$,
we have
\begin{equation}
\begin{aligned}
    L 
    & \geq \frac{\| \mathbf{x} - \mathbf{x}^\ast \|}{2}  * K  \\
    & \geq \frac{\| \mathbf{x} - \mathbf{x}^\ast \|}{2}  * \max_i L_i \\
    & = \frac{\| \mathbf{x} - \mathbf{x}^\ast \|}{2}  * \max_i \max_{\mathbf{x}^\prime\in \mathcal{B}_2(\mathbf{x},\epsilon)} \| H(\mathbf{x}^\prime)_i \|_2.
\end{aligned}
\end{equation}

\noindent \textbf{Extension.}
Notice that
% as long as $\mathbf{x}_s \in B_2(\mathbf{x}_r, \epsilon)$ for small $\epsilon$,
both the lower bound in Eq. (\ref{eq:thickness_lower_bound}) and the upper bounds in Eq. (\ref{eq:thickness_upper_bound}) hold for \textit{any} choice of $\mathbf{x}^\prime = \{ \mathbf{x}^\prime \sim \mathcal{D}: \mathbf{x}^\prime \in \mathcal{B}_2(\mathbf{x}, \epsilon) \}$ with small $\epsilon$.
Thus, 
% $\mathbb{E}_{\mathbf{x}_s} \left[ \int_0^1 h(\mathbf{x}(t),i,j) dt \right]$ is bounded by:
\begin{equation*}
\begin{aligned}
    & h(\mathbf{x},i,j) - 
    \epsilon * \frac{1}{2} \|H(\mathbf{x})_i -H(\mathbf{x})_j\|_2
    \leq \\
    &
    \mathbb{E}_{\mathbf{x}^\prime} 
    \left[ \int_0^1 h(\mathbf{x}(t),i,j) dt
    \right]
    \leq
    % g(\mathbf{x}_r)_i - g(\mathbf{x}_r)_j +
    h(\mathbf{x},i,j) +
    \epsilon * (L_i + L_j).
\end{aligned}
\end{equation*}

Furthermore, 
the bounds of the relaxed local top-$k$ ranking thickness are
\begin{equation}
\begin{aligned}
    & \sum_{i=1}^k \sum_{j=k+1}^n 
    \left[
    h(\mathbf{x},i,j) - 
    \epsilon * \frac{1}{2} \|H(\mathbf{x})_i - H(\mathbf{x})_j\|_2
    \right] \\
    &
    \leq 
    \mathbb{E}_{\mathbf{x}^\prime} 
    \left[ 
    \sum_{i=1}^k \sum_{j=k+1}^n 
    \int_0^1 h(\mathbf{x}(t),i,j) dt
    \right]
    \\ &
    \leq
    \sum_{i=1}^k \sum_{j=k+1}^n 
    \left[
    h(\mathbf{x},i,j) +
    \epsilon * (L_i + L_j)
    \right].
    \label{eq:topk_thick_bound}
\end{aligned}
\end{equation}
 
Even though one can broaden the thickness of \textit{one} ($i,j$) pair by maximizing $\mathcal{I}(\mathbf{x})_i - \mathcal{I}(\mathbf{x})_j$ and 
minimizing $\|H(\mathbf{x})_i -H(\mathbf{x})_j\|_2$ explicitly, 
it is infeasible to minimize $\|H(\mathbf{x})_i -H(\mathbf{x})_j\|_2$ in the top-$k$ thickness case.
Notice that $H(\mathbf{x})_i=H(\mathbf{x})_j, \forall i \in \{1,...\dots,k\},\forall j \in \{k+1,\dots, n\}$ 
indicates
$H(\mathbf{x})_i=H(\mathbf{x})_j, \forall i,j \in \{1,\dots, n\}$,
and we have $H(\mathbf{x})_{iv} = H(\mathbf{x})_{jv}$
where $H(\mathbf{x})_{iv}$ is the element in the $i$-th row and $v$-th column of the Hessian matrix.
For any $i,j,u,v \in \{1,\dots,n\}$,
$H(\mathbf{x})_{iv} = H(\mathbf{x})_{jv} = H(\mathbf{x})_{vj} = H(\mathbf{x})_{uj}$ holds,
which implies that \textit{all} elements in the Hessian matrix of the optimum are the same and results in zero determinant of $H$.
An alternative practical objective is to minimize Hessian norm, $\|H(\mathbf{x})\|$, to tighten the bounds of thickness.

\subsection{Connection between AT and R2ET} 
\label{sec:appendix_connect_at_thickness}
\noindent\textbf{Definition.}
Following the notations used in Sec. \ref{sec:preliminary},
given a model $f:\mathbb{R}^n\to [0,1]^C$ and an input $\bx$,
$\mathcal{I}(\bx,c;f)=\nabla_\bx f(\bx)_c$ is the explanation and $\mathcal{I}(\bx)_i$ is the feature score for the $i$-th feature. 
We further assume that $\mathcal{I}(\bx)$ is sorted and top-$k$ ones are salient features.

We show the following objective of Adversarial Training (AT) for training model over the training set by a min-max game in Sec. \ref{sec:ranking_thickness_defense},
\begin{equation}
\small
\begin{aligned}
\label{eq:obj_at}
    \min_\bw \max_{(\delta_{1,k+1},\dots,\delta_{k,n}) \in \mathcal{N}} 
    \mathcal{L}_{cls}
    - 
    \mathbb{E}_\bx \left[
    \sum_{i=1}^k\sum_{j=k+1}^n h(\bx + \delta_{i,j}, i, j)
    \right],
\end{aligned}
\end{equation}

We start with the one that considers a single sample $\bx$:
\begin{equation}
\label{eq:appendix_at_h_obj}
    \min_\bw \max_{(\delta_{1,k+1},\dots,\delta_{k,n}) \in \mathcal{N}} \mathcal{L}_{cls} - \sum_{i=1}^k \sum_{j=k+1}^n
    h(\bx + \delta_{i,j}, i, j).
\end{equation}
For brevity, 
we consider an auxiliary label:
% $l_i = 2*\mathbbm{1}[i\leq k]-1$. 
$l_i=1$ for $i\leq k$, and $l_i=-1$ otherwise.
and re-write the goal of AT with the auxiliary label $l_i$:
\begin{equation}
    \min_\bw \max_{(\delta_1,\dots,\delta_m)\in\mathcal{N}} \mathcal{L}_{cls} - \sum_{i=1}^m l_i \mathcal{I}(\bx+\delta_i)_i,
\end{equation}
or
\begin{equation}
\label{eq:appendix_at_obj}
    \max_\bw \min_{(\delta_1,\dots,\delta_m)\in\mathcal{N}} - \mathcal{L}_{cls} + \sum_{i=1}^m l_i \mathcal{I}(\bx+\delta_i)_i.
\end{equation}
Notice that $\delta_i$ is specific to the $i$-th feature of input $\bx$.
Based on the definition of $l_i$, 
$\sum_{i=1}^m l_i \mathcal{I}(\bx)_i$ shares the same goal as $\sum_{i=1}^k \sum_{j=k+1}^n h(\bx,i,j)$ but with different weights.

We will start with the inner ($\delta$) part in Eq. (\ref{eq:appendix_at_obj}) and find the connection with R2ET.
We now define an $\epsilon$ norm ball $\mathcal{N}_0 \coloneqq \{\delta: \| \delta \| \leq \epsilon \} \subseteq \mathbb{R}^n$.
We consider a perturbation set $\mathcal{N} \subseteq \mathbb{R}^{n\times n}$
where the perturbations on \textit{each feature} are independently, but the aggregation of perturbations are controlled.
Formally, $\mathcal{N}$ satisfies $\mathcal{N}^- \subseteq \mathcal{N} \subseteq \mathcal{N}^+$ where
\begin{equation*}
\begin{aligned}
    \mathcal{N}^- &  \coloneqq \cup_{i=1}^m \mathcal{N}^-_i; \\
    & \textnormal{where} \quad
    \mathcal{N}^-_i \coloneqq \{ (\delta_1, \dots, \delta_m) | \delta_i \in \mathcal{N}_0; \delta_{t\neq i} = \bm{0} \}. \\
    \mathcal{N}^+ & \coloneqq \{ (\alpha_1\delta_1, \dots, \alpha_m\delta_m) | 
    \sum_{i=1}^n \alpha_i=1; \\
    & \quad \quad \quad \quad \quad \quad \quad
    \alpha_i \geq 0, \delta_i \in \mathcal{N}_0, i=1,\dots,m \}.
\end{aligned}
\end{equation*}
$\mathcal{N}_i^-$ contains $m$ perturbations where only the one pair of features are targeted for a manipulation from $\mathcal{N}_0$ and others are zero vectors.
% $\mathcal{N}^-$ is the union of $\mathcal{N}_i^-$ for each ($i,j$) pair of the $m$ features.
% In $\mathcal{N}^+$, perturbations for all features are considered.

$\mathcal{N}^- \subseteq \mathcal{N} \subseteq \mathcal{N}^+$ naturally indicates that 
\begin{equation}
\label{eq:appendix_inequalities}
\begin{aligned}
    & \min_{(\delta_1,\dots,\delta_m) \in \mathcal{N}^+} \sum_{i=1}^m l_i \mathcal{I}(\bx+\delta_i)_i \\
    \leq 
    & \min_{(\delta_1,\dots,\delta_m) \in \mathcal{N}} \sum_{i=1}^m l_i \mathcal{I}(\bx+\delta_i)_i \\
    \leq 
    & \min_{(\delta_1,\dots,\delta_m) \in \mathcal{N}^-} \sum_{i=1}^m l_i \mathcal{I}(\bx+\delta_i)_i.
\end{aligned}
\end{equation}

% We consider $\mathcal{I}(\bx)_i=\bw_i^\top \bx$.
% We aim to prove that $\min_{(\delta_1,\dots,\delta_n) \in \mathcal{N}} \sum_{i=1}^n l_i \mathcal{I}(\bx+\delta_i)_i$ is equivalent to \textcolor{red}{$\nu=\sum_{i=1}^n l_i \bw_i^\top \bx - \epsilon \max_t \| \bw_t \|$} by proving that $\nu$ is not smaller than the rightmost term and not larger than the leftmost term in Eq. (\ref{eq:appendix_inequalities}).
We approximate $\mathcal{I}(\bx+\delta_i)_i$ by Taylor expansion $\mathcal{I}(\bx+\delta_i)_i=\mathcal{I}(\bx)_i + H(\bx)_i^\top \delta_i$,
where $H(\bx)_i$ is the $i$-th row of Hessian matrix.
We aim to prove that 
\begin{equation}
\label{eq:appendix_delta_n}
    \min_{(\delta_1,\dots,\delta_m) \in \mathcal{N}} \sum_{i=1}^m l_i \mathcal{I}(\bx+\delta_i)_i
\end{equation}
is equivalent to 
\begin{equation}
\label{eq:appendix_nu}
    \nu=\sum_{i=1}^n l_i \mathcal{I}(\bx)_i - \epsilon \max_t \| H(\bx)_t \|_2
\end{equation} 
by proving that $\nu$ is not smaller than the rightmost term and not larger than the leftmost term in Eq. (\ref{eq:appendix_inequalities}).

\noindent \textbf{ To prove $\nu \geq \min_{(\delta_1,\dots,\delta_m) \in \mathcal{N}^-} \sum_{i=1}^m l_i \mathcal{I}(\bx+\delta_i)_i$.}

\begin{equation*}
\begin{aligned}
    & \min_{(\delta_1,\dots,\delta_m) \in \mathcal{N}^-} \sum_{i=1}^m l_i \mathcal{I}(\bx+\delta_i)_i \\
    \leq
    & \min_{(\delta_1,\dots,\delta_m) \in \mathcal{N}_i^-} \sum_{i=1}^m l_i \mathcal{I}(\bx+\delta_i)_i \\
    =
    % & \min_{(\delta_1,\dots,\delta_n) \in \mathcal{N}_i^-} \sum_{i=1}^n l_i \bw_i^\top\bx + l_i \bw_i^\top\delta_i \\
    % =
    % & \sum_{i=1}^n l_i \bw_i^\top \bx + \sum_{i=1}^n \min_{(\delta_1,\dots,\delta_n) \in \mathcal{N}_i^- } l_i \bw_i^\top\delta_i \\
    % =
    % & \sum_{i=1}^n l_i \bw_i^\top \bx + \min_{\delta_t \in \mathcal{N}_0 } l_t \bw_t^\top\delta_t \\
    % = 
    % & \sum_{i=1}^n l_i \bw_i^\top \bx - \epsilon \max_{t} \| \bw_t \|.
    & \min_{(\delta_1,\dots,\delta_m) \in \mathcal{N}_i^-} \sum_{i=1}^m l_i \mathcal{I}(\bx)_i + l_i H(\bx)_i^\top \delta_i \\
    =
    & \sum_{i=1}^m l_i \mathcal{I}(\bx)_i + \sum_{i=1}^m \min_{(\delta_1,\dots,\delta_m) \in \mathcal{N}_i^- } l_i H(\bx)_i^\top \delta_i \\
    =
    & \sum_{i=1}^m l_i \mathcal{I}(\bx)_i + \min_{t\in \{1,\dots, m\} } \min_{\delta_t \in \mathcal{N}_0 } l_t H(\bx)_t^\top \delta_t \\
    = 
    & \sum_{i=1}^m l_i \mathcal{I}(\bx)_i - \epsilon \max_{t \in \{1,\dots, m\} } \| H(\bx)_t \|_2.
\end{aligned}
\end{equation*}
The inequality on line-2 holds since $\mathcal{N}_i^-\subseteq \mathcal{N}^-$.
The equality on line-5 holds due to the definition of $\mathcal{N}_i^-$, where only one $\delta_t$ of $(\delta_1,\dots, \delta_m)$ is from $\mathcal{N}_0$ and the rest are all zeros.
The equality on line-6 holds by picking $\delta_t=-l_t H(\bx)_t$.

\noindent \textbf{ To prove $\nu \leq \min_{(\delta_1,\dots,\delta_m) \in \mathcal{N}^+} \sum_{i=1}^m l_i \mathcal{I}(\bx+\delta_i)_i$.}

\begin{equation*}
\begin{aligned}
    & \min_{(\delta_1,\dots,\delta_m) \in \mathcal{N}^+} \sum_{i=1}^m l_i \mathcal{I}(\bx+\delta_i)_i \\
    =
    & \min_{\sum_i \alpha_i=1, \alpha_i\geq 0, \hat{\delta}_i\in\mathcal{N}_0} \sum_{i=1}^m l_i \alpha_i \mathcal{I}(\bx+\hat{\delta}_i)_i \\
    =
    % & \sum_{i=1}^n l_i \bw_i^\top \bx + \min_{\sum_i \alpha_i=1, \alpha_i\geq 0} \sum_{i=1}^n \alpha_i \min_{\hat{\delta}_i\in\mathcal{N}_0} l_i \bw_i^\top\hat{\delta}_i \\
    % \geq 
    % & \sum_{i=1}^n l_i \bw_i^\top \bx + \min_t \min_{\hat{\delta}_t\in\mathcal{N}_0} l_t \bw_t^\top\hat{\delta}_t \\
    % =
    % & \sum_{i=1}^n l_i \bw_i^\top \bx - \epsilon \max_t \| \bw_t \|.
    & \sum_{i=1}^m l_i \mathcal{I}(\bx)_i + \min_{\sum_i \alpha_i=1, \alpha_i\geq 0} \sum_{i=1}^m \alpha_i \min_{\hat{\delta}_i\in\mathcal{N}_0} l_i H(\bx)_i^\top \delta_i \\
    = 
    & \sum_{i=1}^m l_i \mathcal{I}(\bx)_i + \min_{t \in \{ 1, \dots, m\} } \min_{\hat{\delta}_t\in\mathcal{N}_0} l_t H(\bx)_t^\top \delta_t \\
    =
    & \sum_{i=1}^m l_i \mathcal{I}(\bx)_i - \epsilon \max_{t \in \{ 1, \dots, m\} } \| H(\bx)_t \|_2.
\end{aligned}
\end{equation*}

\noindent \textbf{Connection between AT and R2ET.}
By comparing $ \min_{(\delta_1,\dots,\delta_m) \in \mathcal{N}^-} \sum_{i=1}^m l_i \mathcal{I}(\bx+\delta_i)_i \leq \nu = \min_{(\delta_1,\dots,\delta_m) \in \mathcal{N}^+} \sum_{i=1}^m l_i \mathcal{I}(\bx+\delta_i)_i$ with Eq. (\ref{eq:appendix_inequalities}), 
we could establish the equivalence between
% $\min_{(\delta_1,\dots,\delta_n) \in \mathcal{N}} \sum_{i=1}^n l_i \mathcal{I}(\bx+\delta_i)_i$ and $\nu$.
Eq. (\ref{eq:appendix_delta_n}) and Eq. (\ref{eq:appendix_nu}).
We further add $\mathcal{L}_{cls}$ and taking the maximization over $\bw$ on both terms, 
which indicates that the goal of AT in Eq. (\ref{eq:appendix_at_obj}) is equivalent to 
\begin{equation}
    % \max_\bw -\mathcal{L}_{cls} + \sum_{i=1}^n l_i \bw_i^\top \bx - \epsilon \max_t \| \bw_t \|
    \max_\bw -\mathcal{L}_{cls} + \sum_{i=1}^m l_i \mathcal{I}(\bx)_i - \epsilon \max_t \| H(\bx)_t \|_2,
\end{equation}
or 
\begin{equation}
    \min_\bw \mathcal{L}_{cls} - \sum_{i=1}^m l_i \mathcal{I}(\bx)_i + \epsilon \max_t \| H(\bx)_t \|_2.
\end{equation}
% Recall that $l_i=1$ for $i\leq k$, and $-1$ otherwise.
% The goal of $\sum_{i=1}^n l_i \mathcal{I}(\bx)_i$ is the same as $h(\bx,i,j)=\mathcal{I}(\bx)_i-\mathcal{I}(\bx)_j$ where $i\leq k$ and $j>k$ in Eq. (\ref{eq:defense_thick}) but with different weights.
Notice that these are for one input $\bx$, and $t$ could be different for various $\bx$.
In other words,
$\min_\bw \max_t \| H(\bx)_t \|_2$ will have the same impact as $\min_\bw \|H(\bx) \|_2$ in practice.
In sum,
further replacing $\min_\bw \max_t \| H(\bx)_t \|_2$ by $\min_\bw \|H(\bx) \|_2$ indicates the equivalent between Eq. (\ref{eq:appendix_at_obj}) and
\begin{equation}
\label{eq:appendix_r2et_obj}
    \min_\bw \mathcal{L}_{cls} - \sum_{i=1}^m l_i \mathcal{I}(\bx)_i + \epsilon \| H(\bx) \|_2.
\end{equation}
% In sum, 
% we see that the objective function of R2ET in Eq.(\ref{eq:defense_thick}) is consistent with the goal of AT in Eq. (\ref{eq:appendix_at_obj}).
The equivalence between Eq. (\ref{eq:defense_thick}) and Eq. (\ref{eq:appendix_at_h_obj}) can be proved similarly by replacing $\sum_{i=1}^m l_i \mathcal{I}(\bx)_i$ by $\sum_{i=1}^k \sum_{j=k+1}^n 2h(\bx,i,j)$ and considering all inputs $\bx$ from training set.
% Eq. (\ref{eq:appendix_r2et_obj}) recovers Eq. (\ref{eq:defense_thick}),
% and the proof connecting Eq. (\ref{eq:defense_thick}) and Eq. (\ref{eq:appendix_at_h_obj}) holds.

\subsection{A multi-objective attacking algorithm and its analysis}
We present an algorithm that will terminate in finite iterations, and flip the first pair of salient and non-salient features, or claim a failed attack.
The algorithm is based on a trust-region method designed for single non-convex but smooth objective with nonlinear and non-convex equality constraints~\cite{Cartis2014}.

Let the output vector $f(\bx)=[f_1(\bx),\dots, f_C(\bx)]$.
Given $n$ features and top-$k$ salient features, there are $m=k\times (n-k)$ objectives that can be indexed by subscripts $\ell$ so that the objective vector becomes $[h_1(\bx),\dots,h_\ell(\bx),\dots,h_{m}(\bx)]$.
Let $\|\|$ be a convex norm with Lipschitz constant 1.

Since we are working with numerical algorithms,
an approximately feasible set will be appropriate.
Define the following constrained MOO problem
\begin{equation}
    \label{eq:moo_attack}
    \begin{aligned}[t]
        \min_{\bx}
    	~~ & [h_1(\bx),\dots, h_\ell(\bx),\dots, h_m(\bx)],\\
        \mbox{s.t.} ~~ &
        \|f(\bx) -  f(\bx^{(0)})\| \leq \epsilon_f,\\
        ~~ &
        \|\bx-\bx^{(0)}\|_2 \leq \epsilon_x
    \end{aligned}
\end{equation}
In the following analysis,
we ignore the constraint $\|\bx-\bx^{(0)}\|_2 \leq \epsilon_x$, since it can be combined with the first constraint to obtain a new constraint
\begin{equation}
    \|\tilde{f}(\bx) - \tilde{f}(\bx_0)\|\leq \epsilon,
\end{equation}
for some $\epsilon>0$, with
\begin{equation}
    \tilde{f}(\bx)=[f(\bx), \bx].
\end{equation}
Therefore, we let $f$ denote $\tilde{f}$ to simplify the notation.
Define the domain
\begin{equation}
\label{eq:approx_feasible_set}
\mathcal{C}_1\defeq\{\bx:\|f(\bx)-f(\bx^{(0)})\|\leq \epsilon\}.
\end{equation}

\textbf{Assumption H.1}: \textit{
    The constraint function $f(\bx)$ is continuously differentiable on the domain $\mathbb{R}^n$,
    and the objective functions $h_\ell$, $\ell=1,\dots, m$, are continuously differentiable in the set 
    \begin{equation}
        \mathcal{C}_2\defeq \mathcal{C}_1 + \mathcal{B}(0,\delta \Delta^{(1)}),
    \end{equation}
where $\delta>1$ is a constant, $\Delta^{(1)}$ is the initial radius argument for the trust-region method for multi-objective optimization TR-MOO($\bx,\Delta$) to be defined below, and $\mathcal{B}(0,\delta \Delta^{(1)})$ is an open ball centered at 0 of radius $\delta \Delta^{(1)}$.
}

\textbf{Assumption H.2}: \textit{
    The constraint function $f(\bx)$'s  is continuously differentiable on the domain $\mathbb{R}^n$,
    and the objective functions $h_\ell$, $\ell=1,\dots, m$, are continuously differentiable in the set 
    \begin{equation}
        \mathcal{C}_2\defeq \mathcal{C}_1 + \mathcal{B}(0,\delta \Delta^{(1)}),
    \end{equation}
where $\delta>1$ is a constant, $\Delta^{(1)}$ is the initial radius argument for the trust-region method for multi-objective optimization TR-MOO($\bx,\Delta$) to be defined below, and $\mathcal{B}(0,\delta \Delta^{(1)})$ is an open ball centered at 0 of radius $\delta \Delta^{(1)}$.
}

\textbf{Assumption H.3}: \textit{
    The objective functions $h_\ell$, $\ell=1,\dots, m$ are bounded below and above in the set $\mathcal{C}_1$. More specifically,
}
    \begin{align}
    h_{\textnormal{low}}&\defeq\min_\ell\{\min_\bx h_1(\bx),\dots, \min_\bx h_m(\bx)\}, \\
h_{\textnormal{up}} & \defeq\max_\ell\{\max_\bx h_1(\bx),\dots, \max_\bx h_m(\bx)\}.
    \end{align}

We give an attacking algorithm MOO-attack below that can either find the first feature pair to flip in an explanation, or to claim that it is impossible to flip any feature pair.
In the algorithm, superscript $(k)$, $k=1,2,\dots$ indicates the number of iterations.
\begin{algorithm}
\setstretch{1}
\caption{Attacking a pair of features}
\begin{algorithmic}
    \STATE \textbf{Input}: initial input $\bx$, target model $f$, current explanation $\mathcal{I}(\bx)$, tolerance $\epsilon>0$, trust-region method parameters $1>\eta>0$ and $1>\gamma>0$.
    \STATE Set $k=1$, $\bx^{(k)}=\bx$, $t_\ell^{(k)}=\|f(\bx^{(k)})\|+h_\ell(\bx^{(k)})-\epsilon^{(k)}$ for each objective $h_\ell$.
    \WHILE{$\min_{1\leq \ell\leq m} \chi_\ell(\bx^{(k)},t^{(k)}) \geq \epsilon$}
    \STATE Solve TR-MOO$(\bx^{(k)},\Delta^{(k)})$ to obtain a joint descent direction $\mathbf{d}^{(k)}$ for all linearized merit functions $l_{\phi_{\ell}}$.
    \STATE $\rho_\ell^{(k)}=\frac{\phi_\ell(\bx^{(k)},t^{(k)})-\phi_\ell(\bx^{(k)}+d^{(k)},t^{(k)})}{l_{\phi_{\ell}}(\bx^{(k)}, t_\ell^{(k)}, 0) - l_{\phi_{\ell}}(\bx^{(k)}, t_\ell^{(k)}, \mathbf{d}^{(k)})}$ for each $\ell=1,\dots, m$.
    \IF{$\min_\ell \rho_\ell^{(k)}>\eta$}
        \STATE $\bx^{(k+1)}=\bx^{(k)}+\mathbf{d}^{(k)}$.
        \STATE $\Delta^{(k+1)}=\Delta^{(k)}$.
        \IF{$h_\ell(\bx^{(k)})\geq t_\ell^{(k)}$}
        \STATE $t_\ell^{(k+1)}=t_\ell^{(k)}-\phi_\ell(\bx^{(k)},t_\ell^{(k)})+\phi_\ell(\bx^{(k+1)},t_\ell^{(k)})$.
        \ELSE
        $t_\ell^{(k+1)}=2h_\ell(\bx^{(k+1)})-t^{(k)}-\phi_\ell(\bx^{(k)},t_\ell^{(k)})+\phi_\ell(\bx^{(k+1)},t_\ell^{(k)})$.
        \ENDIF
    \ELSE
        \STATE $\bx^{(k+1)}=\bx^{(k)}$.
        \STATE $\Delta^{(k+1)}=\gamma\Delta^{(k)}$.
        \STATE $t_\ell^{(k+1)}=t_\ell^{(k)}$ for $\ell=1,\dots,m$.
    \ENDIF
    \ENDWHILE
\end{algorithmic}
\label{alg:moo_attack}
\end{algorithm}

TR-MOO$(\bx,\Delta)$:
\begin{equation}
    \left\{
    \begin{array}{cl}
         \min_{\alpha,\mathbf{d}} & \alpha   \\
        \textnormal{s.t.} & l_{\phi_{\ell}}(\bx,t,\mathbf{d})\leq \alpha, \ell=1,\dots, m,\\
        & \|\mathbf{d}\|\leq \Delta.
    \end{array}
    \nonumber
    \right.
\end{equation}

The attacking algorithm may not be able to flip any pair of features when $\min_{1\leq \ell\leq m} \chi_\ell(\bx^{(k)},t^{(k)}) < \epsilon$, but there can be other objective functions that still have $\chi_\ell(\bx^{(k)},t^{(k)}) \geq \epsilon$ and there is a chance to flip the corresponding pairs of features. We will remove any objective function $h_\ell$ with $\chi_\ell(\bx^{(k)},t^{(k)}) < \epsilon$ and return to the while loop to try to flip other pairs of features.
If all objective functions are removed at the end, the attacker fails to attack the explanation.

We adapt the theoretical results from~\cite{Cartis2014} to the above multi-objective optimization algorithm to show a global convergence rate for the attacker.

First, the following lemma shows sufficient descent in the linearized merit functions in the direction $\mathbf{d}^{(k)}$.
\begin{lemma}
\label{lem:suff_reduced}
Suppose that assumption A.1 holds. If $\bx^{(k)}\in \mathcal{C}_1$ defined in Eq. (\ref{eq:approx_feasible_set}),
then 
\begin{eqnarray}
\label{eq:merit_func_linear_reduction}
    &l_{\phi_{\ell}}(\bx^{(k)}, t_\ell^{(k)}, 0) - l_{\phi_{\ell}}(\bx^{(k)}, t_\ell^{(k)}, \mathbf{d}^{(k)})\nonumber\\
    &\geq \min(\Delta^{(k)},1)\chi_\ell(\bx^{(k)}, t^{(k)}),
\end{eqnarray}
for each linearized merit function $l_{\phi_\ell}$ defined in Eq. (\ref{eq:merit_func_linear}).
\end{lemma}
The proof can be found in Lemma 2.1 in~\cite{Cartis2014}.

The next lemma shows that from iteration to iteration during the while loop in Algorithm~\ref{alg:moo_attack}, the following invariant will be maintained.
\begin{lemma}
\label{lem:invariant}
Suppose that assumption A.1 holds.
In each iteration for $k\geq 1$ in Algorithm~\ref{alg:moo_attack},
the following properties hold:
\begin{equation}
    h_\ell(\bx^{(k)}) - t_\ell^{(k)} > 0, \ell=1,\dots, m,
\end{equation}
\begin{equation}
    \phi_\ell(\bx^{(k)}, t_k) = \epsilon, \ell=1,\dots, m,
\end{equation}
\begin{equation}
    |h_\ell(\bx^{(k)}) - t_\ell^{(k)}| \leq \epsilon, \ell=1,\dots, m,
\end{equation}
\begin{equation}
    \|f(\bx^{(k)})\| \leq \epsilon.
\end{equation}
\end{lemma}
The proof can be obtained via applying Lemma 2.2 in~\cite{Cartis2014} to each of the objective functions independently.

The last inequality indicates that during the attack, the manipulated input $\bx^{(k)}$ remains in the approximate feasible set $\mathcal{C}_1$ and that the prediction by $f$ is not changed. This is important to make the attack stealthy.
The second last inequality shows that each objective $h_\ell$ will chase the corresponding target $t_\ell^{(k)}$ over the iterations, so that if $t_\ell^{(k)}$ can be shown to be decreasing sufficiently fast, we can show the convergence of $h_\ell$.
Note that different targets $t_\ell^{(k)}$ will move in different speed, as they are updated independently in the algorithm. Also, a target is not guarantee to be reduced below zero for $h_\ell$ to become negative and the $\ell$-th pair of features will be flipped.

The next lemma shows that when the radius $\Delta^{(k)}$ used in TR-MOO($\mathbf{x}^{(k)}$, $\Delta^{(k)}$) is small enough, the radius won't be further reduced. Together with Lemma~\ref{lem:suff_reduced}, the linearized merit functions are reduced sufficiently per iteration.
\begin{lemma}
Suppose that assumptions A.1 and A.2 hold. Then with $\min_{\ell}\chi_{\ell}(\bx^{(k)},t^{(k)})\geq \epsilon$ and
\begin{equation}
     \Delta^{(k)}\leq \min_\ell\frac{(1-\eta)\epsilon}{L_{g_\ell} + \frac{1}{2}L_J},
\end{equation}
we will have the condition $\min_\ell \rho_\ell^{(k)}>\eta$ in Algorithm~\ref{alg:moo_attack} hold true and $\Delta^{(k+1)}=\Delta^{(k)}$.
Further more, with $\min_{\ell}\chi_{\ell}(\bx^{(k)},t^{(k)})\geq \epsilon$,
we have, for all $k\geq 1$,
\begin{equation}
\label{eq:lb_of_Delta}
    \Delta^{(k)}\geq \textnormal{min}\left(\Delta^{(1)}, \min_{\ell}\frac{(1-\eta)\gamma}{L_{g_\ell}+\frac{1}{2}L_J}\right)\epsilon.
\end{equation}
\end{lemma}
The proof is a modification to the proof of Lemma 3.2 in~\cite{Cartis2014},
with the derivation done for each of the objective function $h_\ell$ to guarantee sufficient descent in all merit functions.
An interesting observation is that the search radius $\Delta^{(k)}$ is restricted by the objective that has the most rapid change in its gradient $g_\ell$ (characterized by $L_{g_\ell}$). If all objectives are smooth (with small $L_{g_\ell}$), the search radius can be larger and reduction in the merit functions is larger.
The second inequality of the above lemma says that the search radius will have a lower bound across all iterations.

How many times do we need to reduce the search radius is characterized in the following lemma.
\begin{lemma}
    There are at most $O(\lceil |\log(\epsilon)|\rceil)$ number of times that $\Delta^{(k)}$ will be reduced by the factor of $\gamma$.
\end{lemma}
That is because, starting from $\Delta^{(1)}$,
once $\Delta^{(k)}$ falls below $\min_\ell\frac{(1-\eta)\epsilon}{L_{g_\ell} + \frac{1}{2}L_J}$ at iteration $k$,
there will be no more reduction in future iterations.

The following lemma show sufficient reduction in the merit functions and the targets.
\begin{lemma}
\label{lem:suff_reduction_target}
Suppose that assumptions A.1 and A.2 hold.
Whenever $\bx^{(k)}$ is updated in Algorithm~\ref{alg:moo_attack},
for each objective function $h_\ell$,
both the reductions 
$\phi_\ell(\bx^{(k)},t_\ell^{(k)},0)
    -\phi_\ell(\bx^{(k)},t_\ell^{(k)},\mathbf{d}^{(k)})$
and $t_\ell^{(k)}-t_\ell^{(k)}$ are at least
\begin{equation}
    \textnormal{min}\left(\Delta^{(1)}, \min_{\ell}\frac{(1-\eta)\gamma}{L_{g_\ell}+\frac{1}{2}L_J}\right)\epsilon^2\eta.
\end{equation}
\end{lemma}
The proof is to use the condition that $\rho_\ell^{(k)}>\eta$ for all $\ell=1,\dots, m$, Eq. (\ref{eq:merit_func_linear_reduction}), the condition that $\min_{1\leq \ell\leq m} \chi_\ell(\bx^{(k)},t^{(k)}) \geq \epsilon$, and Eq. (\ref{eq:lb_of_Delta}).

Lastly, we present the main global convergence results.
Let $h_{\textnormal{low}}\defeq\min_\ell\{\min_\bx h_1(\bx),\dots, \min_\bx h_m(\bx)\}$ and 
$h_{\textnormal{up}}\defeq\max_\ell\{\max_\bx h_1(\bx),\dots, \max_\bx h_m(\bx)\}$.
\begin{theorem}
Suppose assumptions A.1-A.3 hold.
Then Algorithm~\ref{alg:moo_attack} generates an $\epsilon-$first-order critical point for problem Eq. (\ref{eq:moo_attack}) in at most
\begin{equation}
    \Bigl\lceil\left(h_{\textnormal{up}}-h_{\textnormal{low}}\right)\frac{\kappa}{\epsilon^2}\Bigr\rceil
\end{equation}
iterations of the while loop in the algorithm, where $\kappa$ is a constant independent of $\epsilon$ but depending on $\gamma$, $\eta$, $L_{h_\ell}$, and $L_J$.
\end{theorem}
The proof hinge on the following inequality
\begin{align}
h_{\textnormal{low}} &\leq h_\ell(\bx^{(k)})\\
&\leq t_\ell^{(k)}+\epsilon\\
&\leq t_\ell^{(1)} - i_k \kappa_2 \epsilon^2 + \epsilon\\
&\leq h_\ell(\bx^{(1)})- i_k \kappa_2 \epsilon^2  + \epsilon\\
&\leq h_{\textnormal{up}}- i_k \kappa_2 \epsilon^2  + \epsilon
\end{align}
where $i_k$ is the number of iterations between 1 and $k$ where $\min_\ell \rho_\ell^{(k^\prime)}>\eta$, $1\leq k\leq k^\prime$, is true.
\begin{equation}
    \kappa_2=\textnormal{min}\left(\Delta^{(1)}, \min_{\ell}\frac{(1-\eta)\gamma}{L_{g_\ell}+\frac{1}{2}L_J}\right)\eta.
\end{equation}
Therefore,
\begin{equation}
    i_k\leq \Bigl\lceil\frac{h_{\textnormal{up}}-h_{\textnormal{low}}+\epsilon}{\kappa_2\epsilon^2}\Bigr\rceil.
\end{equation}

Since $O(\lceil|\log(\epsilon)|\rceil)$ grows slower than $1/\epsilon^2$, the overall number of iterations is in the order of  $\Bigl\lceil\left(h_{\textnormal{up}}-h_{\textnormal{low}}\right)\frac{\kappa}{\epsilon^2}\Bigr\rceil$.

\textbf{Comments:}
\begin{itemize}
    \item
If after the while loop, no $h_\ell$ is reduced to a negative value, then one remove those $h_\ell$ that has reached the approximate critical point and continue the while loop with the remaining objective functions.
The next while loop starts with a smaller gap $h_{\textnormal{up}}-h_{\textnormal{low}}$ defined over the remaining objectives.
Since there are a finite number of objectives, the algorithm finishes in finite iterations.
\item The constraint $\|f(\bx)-f(\bx^{(0)})\|\leq \epsilon$ is maintained over all iterations and thus stay stealthy during the attack.
\end{itemize}
% \section{Reproducibility Checklist: More Experimental Details}
\section{Details of Experiments}
\label{sec:append_experiments}
This section provides more details about the experimental settings and additional results, 
as supplementary for Sec. \ref{sec:experiemnt_whole_section}.

\subsection{Training with R2ET}
\begin{algorithm}
\caption{Training a model with robust ranking explanation by R2ET.}
\label{alg:r2et}
% \hspace*{\algorithmicindent} 
\textbf{Input:} 
Training set $(\mathcal{X}_T,\mathcal{Y}_T)$ and validation set $(\mathcal{X}_V,\mathcal{Y}_V)$; $k$ as number of features of interest; hyperparameter $\lambda_1>0, \lambda_2>0$. \\
% \textbf{Output:} 
% A robust ranking explanation model $f(\bw)$.\\
\begin{algorithmic}[1]
\IF {exists a pretrain model $f_{pre}$}
    \STATE $f(\bw) \gets f_{pre}$
\ENDIF
\FOR{$iteration \leq MaxIter$}
    \STATE calculate $\mathcal{L}_{total}$ of R2ET by Eq. (\ref{eq:defense_thick})
    \STATE $\bw \gets \bw - \eta \nabla \mathcal{L}_{total}$
    \IF {eval ($f, \mathcal{X}_V,\mathcal{Y}_V$) gets better}
    \STATE save model $f(\bw)$ to file
    \ENDIF
\ENDFOR
\STATE load and output model $f(\bw)$ from file
\end{algorithmic}
\end{algorithm}

Algorithm \ref{alg:r2et} provides a way to train the model with R2ET.

\subsection{Datasets}
Our experiments use two types of network architectures: single-input DNNs and dual-input SNs.
For single-input DNNs, we use three tabular datasets, Adult, 
Bank \cite{moro2014data} and COMPAS 
% \cite{chen2021self}.
\cite{mothilal2020explaining}.
We divide each tabular dataset into training, validation and test portions at a ratio of $70:15:15$, respectively.
The original tabular datasets contain a mixture of strings and floating numbers.
Thus, 
we binarize them and map them to 28-dim, 18-dim, and 16-dim feature spaces, respectively \cite{chen2021self}.
We also conduct experiments on CIFAR-10 \cite{krizhevsky2009learning} with ResNet,
where the training set is further divided into the training and validation portion with a ratio of $80:20$.
For dual-input SNs, we use one image dataset, MNIST \cite{lecun1998gradient}, and two graph datasets, BP\cite{ma2019deep} and ADHD.
Using the image dataset MNIST, 
we randomly select 2,400 pairs of images with digits \textit{3} and \textit{8} from training images as the training set, 
and 300 and 600 pairs from test images as the validation and test sets, respectively.
BP and ADHD are graph data consisting of 82 and 116 nodes for the human brain datasets, 
respectively.
Due to the scarcity of graphs for both, 
we use five-fold cross-validation and each time use three of them as training graphs and the other two as validation and test graphs,
respectively. 
We pair any two training graphs as the training set.
To simulate real medical diagnosis (by comparing a new sample with those in the database), 
each pair consists of a training graph and a validation graph as a validation set.
Additionally, each validation graph is paired with two training graphs,
one from the same class and one from a different class.
% Eventually,
% the numbers of positive pairs (two samples from the same class) and negative pairs are the same.
The test set adopts the same setting.
% Besides,
% in image and graph datasets, 
% original inputs are represented in matrices,
% and we flatten images and the upper triangle of the adjacency matrices to vectors,
% such that all types of inputs take the form of $\mathbf{x}\in\mathbb{R}^n$.

\subsection{Evaluation Metrics}
\label{sec:append_metric}
For the target sample $\mathbf{x}$ and the corresponding adversarial sample $\mathbf{x}^\prime=\mathbf{x}+\delta$, 
we evaluate the robustness of ranking explanations by measuring the similarity between explanations,
% $\mathbf{m}=
$\mathcal{I}(\mathbf{x}) \in \mathbb{R}^n$ and 
% $\mathbf{n}=
$\mathcal{I}(\mathbf{x}^\prime) \in \mathbb{R}^n$, 
% and both explanations can be expressed as a vector of length $ n $.
To quantify the \textit{similarity}, we use the following 
% three 
metrics,
\begin{itemize}[leftmargin=*]
    \item \textbf{Precision@$k$ (P@$k$).} 
    Precision@$k$ is widely used to evaluate the similarity between rankings \cite{ghorbani2019interpretation,wang2020smoothed}. 
    P@$k$ is defined by
    % Since in many settings, 
    % only the most important features in an explanation map are of interest, 
    % it is natural to calculate the size of intersection of the $ k $ most important features of two explanations and thus measure their similarity. 
    % To make the metric more intuitive, 
    % we use the top-$ k $ intersection ratio defined as
    % $ \frac{\sum_{i=1}^{k}\frac{1}{i}|T_{i\mathbf{u}} \cap T_{i\mathbf{v}}| }{k} $, 
    \begin{equation*}
        \textnormal{P@$k$}(\mathcal{I}(\mathbf{x}), \mathcal{I}(\mathbf{x}^\prime)) 
        = \frac{ | \mathcal{I}(\mathbf{x})_{[k]} \cap \mathcal{I}(\mathbf{x}^\prime)_{[k]} | }{k},
    \end{equation*} 
    where $ \mathcal{I}(\mathbf{x})_{[k]}$ is the set of the $k$ most important features of the explanation $ \mathcal{I}(\mathbf{x})$.
    $|\cdot|$ counts the number of elements in the intersection of two top $k$ features.
    
%     \item \textbf{Pearson correlation coefﬁcient (PCC).} 
%     Following existing work \cite{dombrowski2019explanations},
%     we also evaluate the similarity of two explanations by Pearson correlation coefficient,
%     \begin{equation*}
%     	{\rm PCC}(\mathcal{I}(\mathbf{x}), \mathcal{I}(\mathbf{x}^\prime))
%     	= 
%     	 \frac{\sum_{i}^{n}(\mathcal{I}(\mathbf{x})_i - \mu(\bx)) (\mathcal{I}(\mathbf{x}^\prime)_i - \mu(\bx^\prime))}
%     % 	{\sqrt{\sum_{i}^{n}(\mathcal{I}(\mathbf{x})_i - \mu)^2} 
%     % 	 \sqrt{\sum_{i}^{n}(\mathcal{I}(\mathbf{x}^\prime)_i - \mu^\prime)^2}}
%         {\sqrt{\sigma(\bx) \sigma(\bx^\prime)}}, 
%     \end{equation*}
%     where $\sigma(\bx)={\sum_{i}^{n}(\mathcal{I}(\mathbf{x})_i - \mu(\bx))^2}$, and $ \mu (\bx) = \frac{1}{n} \sum^n_i \mathcal{I}(\bx)_i$.

% 	\item \textbf{Mean squared error (MSE).} 
% 	We also use the mean squared error to measure the similarity between two explanation maps \cite{dombrowski2019explanations,dombrowski2021towards}, 
% 	\begin{equation*}
% 		{\rm MSE}(\mathcal{I}(\mathbf{x}), \mathcal{I}(\mathbf{x}^\prime)) = \frac{1}{n}\sum_{i}^{n}(\mathcal{I}(\mathbf{x})_i-\mathcal{I}(\mathbf{x}^\prime)_i)^2.
% 	\end{equation*}
\end{itemize}

Besides robustness, 
we use the following metrics to evaluate the model's \textit{classification performance}. 
Related discussion and results can be found in Appendix \ref{sec:constrained_opt_appendix} and \ref{sec:acc_robust_trade_off}.
% from a defender's perspective,
\begin{itemize}[leftmargin=*]
    \item \textbf{Clean AUC (cAUC) and adversarial AUC (aAUC). } 
    An explanation-robust model should also have robust classification performance, 
    so we use the metric cAUC and aAUC to measure the model's classification performance before and after the attack, respectively.
    
    \item \textbf{Sensitivity (Sen).}
    % Since some existing works can detect 
    Since adversarial attacks can be detected by checking the consistency of predictions \cite{xu2020adversarial},
    % models that can make it more difficult for the perturbed sample to keep the original prediction are more conducive for defenders to detect the attack. 
    we use Sen to measure the ratio at which the predicted classification of the perturbed sample changes. 
    More specifically, Sen measures the ratio at which classification result changes after an attack for single-input DNNs. 
    For dual-input SNs, there are three classification results for a pair of samples: 
    one similarity classification result and two classification results from the classifier with respect to two samples,
    respectively. 
    Thus, Sen for SNs measures the ratio at which \textit{any} of three classification results change after attacks.
    
\end{itemize}

We consider three widely adopted metrics to evaluate the \textit{faithfulness} of explanations.
The numerical results can be found in Table \ref{tab:faithfulness}.
\begin{itemize}[leftmargin=*]
    \item \textbf{Decision Flip - Fraction of Tokens (DFFOT)} \cite{serrano2019attention} measures the minimum fraction of important features to be removed to flip the prediction.
    A \textit{lower} DFFOT indicates a more faithful explanation.
    Formally,
    \begin{equation*}
    \begin{aligned}
    & \textnormal{DFFOT} = \min_k \frac{k}{n}, \\
        % \quad 
        & \textnormal{s.t.}
        \quad
        \argmax_c f(\bx)_c \neq \argmax_c f(\bx_{[\backslash k]})_c,
    \end{aligned}
    \end{equation*}
    where $n$ is the number of features, and $\bx_{[\backslash k]}$ is the perturbed input whose top-$k$ important features are removed.
    
    \item \textbf{Comprehensiveness (COMP)} \cite{deyoung2019eraser} 
    measures the changes of predictions before and after removing the most important features.
    A \textit{higher} COMP means a more faithful explanation. Formally,
    \begin{equation*}
        \textnormal{COMP} = \frac{1}{\|K\|} \sum_{k\in K} |f(\bx)_c - f(\bx_{[\backslash k]})_c |,
    \end{equation*}
    where $K$ is $\{1,\dots,n\}$ for tabular data, 
    and  $\{1\% *n, 5\% *n, 10\% *n, 20\% *n, 50\% *n\}$ for images and graphs.
    
    \item \textbf{Sufficiency (SUFF)} \cite{deyoung2019eraser}
    measures the change of predictions if only the important tokens are preserved.
    A \textit{lower} SUFF means a more faithful explanation.
    Formally,
    \begin{equation*}
        \textnormal{SUFF} = \frac{1}{\|K\|} \sum_{k\in K} |f(\bx)_c - f(\bx_{[k]})_c |,
    \end{equation*}
    where $\bx_{[k]}$ is the perturbed input with only top-$k$ important features, 
    and $K$ is set the same as the one for COMP.
\end{itemize}

% we also evaluate the sensitivity that the likelihood of attackers being caught % by defenders.
% The sensitivity is defined by the ratio of samples satisfying three % constraints in Eqs. (\ref{eq:attack_sne_con1})-(\ref{eq:attack_sne_con3}). 
% Otherwise, the defender catch the attackers by checking whether predictions % change before and after attacks.
% To evaluate the effect of Algorithm \ref{alg:attack} on the constraints
% in Eqs. (\ref{eq:attack_sne_con1})-(\ref{eq:attack_sne_con3}). 
% The sensitivity metric is defined by the ratio of attackers being caught by defenders.
% classification results 
% in the three constraints 
% that do not change before and after the attack, 
% and can therefore be used to simulate the probability that the attack will not be detected by the defender.

\subsection{Compared Methods}

We conduct two different attacks,
\textbf{MSE attack} and \textbf{ERAttack}.
MSE attack tries to find the optimal perturbation such that $\|\mathcal{I}(\mathbf{x}), \mathcal{I}(\mathbf{x}^\prime) \|_2^2 $ 
% the MSE between $\mathcal{I}(\mathbf{x})$ and $\mathcal{I}(\mathbf{x}^\prime)$ 
can be maximized.
ERAttack is conducted based on Eq. (\ref{eq:attack_thick}) to manipulate the explanation rankings and more details are in Appendix \ref{sec:general_settings}.

\noindent \textbf{Baselines.}
We compare our proposed methods
% based on ranking-specific defense strategies 
with other state-of-the-art methods under the two attacks mentioned above. 
For simplicity, 
we denote the Hessian matrix of a neural network $ f $ with respect to the input $ \mathbf{x} $ as $ H(\mathbf{x})$.
Authors in \cite{dombrowski2021towards,wang2020smoothed} deduced that the bound on $ \|H(\mathbf{x}) \|_2 $ affects explanation robustness regarding $\ell_p$-norm based manipulations. 
% Motivated by this idea, 
% the following methods make the explanations more robust by directly or indirectly reducing 
% $ \|H(\mathbf{x})\|_2 $:
\begin{itemize}[leftmargin=*]
    \item \textbf{Vanilla}:
    It provides the basic ReLU model that is trained without any robust strategies.
    The other baselines share the same structure with Vanilla model,
    but use weight decay, 
    distinct activation functions, 
    or extra regularizers.
    The structure of Vanilla models is in Appendix \ref{sec:structure_vanilla_model}.
    \item \textbf{Weight Decay (WD)} \cite{dombrowski2021towards}:
    % Since $ \|H(\mathbf{x}) \|_2 $ depends on the weights of the model $ f $, 
    Weight decay during training models is supposed to
    % a method that can be used to effectively 
    improve the explanation robustness by decreasing the weights of the neural networks.
    % as well as the Hessian norm.
    \item \textbf{Softplus (SP)} \cite{dombrowski2019explanations,dombrowski2021towards}:
    % The Softplus activation function, 
    $\textnormal{Softplus}(x;\rho)=\frac{1}{\rho}\ln(1+e^{\rho x})$
    can be regarded as a smooth version of ReLU, 
    and a smaller $ \rho $ results in a smoother curvature.
    Since $ \|H(\mathbf{x})\|_2 $ also depends on the maximal values of the activation function's first and second derivatives, 
    Softplus is used to improve the explanation robustness by virtue of its maximal derivatives being smaller than ReLU's. 
    \item \textbf{Exact-Hessian (Exact-H)}:
    Considering Hessian norm as the regularization during training is a straightforward way to reduce the norm of the Hessian.
    Specifically,
    \begin{equation}
        \min_{\bw} \mathcal{L}_{total} = \mathcal{L}_{cls} (f(\mathbf{x},\bw)) + \lambda \mathbb{E}_{\mathbf{x}\in\mathcal{X}_T}
        \|H(\mathbf{x})\|_2.
    \end{equation}
    Since $ \|H(\mathbf{x})\|_2 $ is calculated exactly for each training set sample $ \mathbf{x} \in \mathcal{X}_T $, 
    this method is denoted as exact-Hessian.
    Notice that 
    it is usually infeasible to explicitly calculate the Hessian matrix nor its Frobenius norm,
    especially for datasets with high-dimensional samples,
    thus it is only used on three tabular data.
    \item \textbf{Estimate-Hessian (Est-H)} \cite{dombrowski2021towards}:
    % Since directly computing the norm of Hessian matrix is very time-consuming, 
    % the method exact-Hessian is only suitable for datasets with few features. 
    As mentioned above, 
    exact-Hessian is very time-consuming due to the explicit computation of Hessian norm.
    In order to apply it to high-dimensional datasets such as images and graphs, 
    we use the finite difference to approximate Hessian norm \cite{pearlmutter1994fast}:
    % \begin{equation}
        % \mathbb{E}_{\mathbf{x}_r\in\mathcal{X}_T} 
        % \| H(\mathbf{x})\mathbf{v} \|_2 
        % \approx
        % \mathbb{E}_{\mathbf{x}_r\in\mathcal{X}_T} 
        $\| \frac{\nabla f(\mathbf{x} + \kappa \mathbf{v}) - \nabla f(\mathbf{x})}{\kappa}\|_2$,
    % \end{equation}
    where $ \kappa \ll 1 $ denotes the discretization step and $ \mathbf{v} $ can be any vector, 
    in practice we set $ \mathbf{v}=\frac{\textnormal{sign}(\nabla f(\mathbf{x}))}
    {\|\textnormal{sign}(\nabla f(\mathbf{x}))\|_2} $ the same as \cite{moosavi2019robustness}.
    \item
    \textbf{SSR} \cite{wang2020smoothed}:
    sets the largest eigenvalue of the Hessian matrix as the regularization.
    \item
    \textbf{Adversarial Training (AT)} 
    % \cite{huang2015learning,shaham2018understanding}: 
    \cite{huang2015learning,wong2020fast}:
    trains the model following a minimization-maximization approach, e.g.,
    \begin{equation*}
    \begin{aligned}
    \min_{f} &
    \sum_{(\mathbf{x},y)\in(\mathcal{X}_T,\mathcal{Y}_T)}
    (\mathcal{L}_{cls} (f;\mathbf{x}+\delta^\ast, y)), \\
    \textnormal{s.t.} & \quad
    \delta^\ast = \argmax_\delta - \sum_{i=1}^k \sum_{j=k+1}^n
    h(\mathbf{x}+\delta, i,j).
    \end{aligned}
    \end{equation*}
\end{itemize}

\noindent \textbf{Proposed methods.}
Based on the defense strategy of maximizing ranking thickness in Sec. \ref{sec:ranking_thickness_defense}, 
we propose the following methods to enhance ranking explanations robustness:
\begin{itemize}[leftmargin=*]
    \item \textbf{Robust Ranking Explanation via Thickness (R2ET)}:
    trains model with Eq. (\ref{eq:defense_thick}) as the objective function to improve the ranking explanation thickness.
    % As mentioned in Sec. \ref{sec:ranking_thickness_def},
    % We replace the indicator function with a differentiable monotonically increasing function of $h$ such as $h(\mathbf{x},i,j)$ itself or $\exp\{h(\mathbf{x},i,j)\}$.
    We try $h(\mathbf{x},i,j)=\mathcal{I}(\mathbf{x})_i - \mathcal{I}(\mathbf{x})_j$ 
    and $h(\mathbf{x},i,j) 
    = \exp{ \{\mathcal{I}(\mathbf{x})_i - \mathcal{I}(\mathbf{x})_j\} }$.
    In practice,
    we find that the exponential version benefits from a non-negative range of functions.
    We try both and present the results from the better ones,
    and similar for the variants of \textbf{R2ET}.
    % This method combines tx/etx and Hessian-related methods (exact-Hessian and est-Hessian), and the loss function can be expressed as
    % \begin{equation}
    % \label{eq:tx/etx+Hessian}
    %           \mathcal{L}_{total} = \mathcal{L}_{cls} (f;\mathcal{X}_T, \mathcal{Y}_T) + \lambda_1 \mathbb{E}_{\mathbf{x}_r\in\mathcal{X}_T} \mathcal{L}_{\textnormal{tx/etx}}(\mathbf{x}_r)
    %       + \lambda_2 \mathbb{E}_{\mathbf{x}_r\in\mathcal{X}_T} \mathcal{L}_{\textnormal{Hessian}}(\mathbf{x}_r), 
    % \end{equation}
    % where $ \lambda_1 $ and $ \lambda_2 $ are balancing hyperparameters.
    
    \item \textbf{R2ET-mm}:
    An alternative selection of comparison pairs is proposed in Sec.  \ref{sec:ranking_thickness_defense}.
    $k^\prime$ distinct indices of $i,j$ will be selected, 
    where $i$ covers the smallest $k^\prime$ features in the top-$k$,
    and $j$ covers the largest $k^\prime$ features in the rest.
    In other words,
    $\sum_{i,j} h(\mathbf{x},i,j)$ for $k^\prime$ pairs is minimized by such selection.
    % This method replaces $ \mathcal{L}_{\textnormal{tx/etx}}(\mathbf{x}_r) $ in Eq. \ref{eq:tx/etx+Hessian} with $ \mathcal{L}_{\textnormal{tx-mm}}(\mathbf{x}_r) $ or $ \mathcal{L}_{\textnormal{etx-mm}}(\mathbf{x}_r) $, leaving the rest unchanged.
    We set $k^\prime=k$ by default, 
    and we study the sensitivity of $k^\prime$ in Appendix \ref{sec:sensitivity_analysis_experiments}.

    \item \textbf{R2ET}$_{\backslash \mathbf{H}}$:
    It serves as the ablation variant of \textbf{R2ET} by setting $\lambda_2=0$ in Eq. (\ref{eq:defense_thick}).
    It strives to broaden the gaps between feature importance directly,
    and does not care about the curvature.
    Notice that \textbf{Est-H} can be considered another ablation variant of \textbf{R2ET} with $\lambda_1=0$.
    % This method uses the acceleration strategy mentioned at the end of Sec. \ref{sec:ranking_thickness_defense} to implement the loss function in Eq. \ref{eq:defense_thick}:
    % \begin{equation}
    % \label{eq:tx}
    % \begin{array}{cc}
    %      &      \mathcal{L}_{total} = \mathcal{L}_{cls} (f;\mathcal{X}_T, \mathcal{Y}_T) + \lambda \mathbb{E}_{\mathbf{x}_r\in\mathcal{X}_T} \mathcal{L}_{\textnormal{tx}}(\mathbf{x}_r),\\
    %      &  \textnormal{where }  \mathcal{L}_{\textnormal{tx}}(\mathbf{x}_r)=-
    %     (\sum_{i=1}^{k-1} h(\mathbf{x}_r, i,k) + \sum_{j=k+1}^{2k} h(\mathbf{x}_r, k,j)).
    % \end{array}
    % \end{equation}
    % In order to make the penalty term non-negative and maximize the ranking thickness while minimizing the total loss, another method is to rewrite $ \mathcal{L}_{\textnormal{tx}}(\mathbf{x}_r) $ as an exponential function:
    % \begin{equation}
    % \label{eq:etx}
    % \begin{array}{cc}
    %      &      \mathcal{L}_{total} = \mathcal{L}_{cls} (f;\mathcal{X}_T, \mathcal{Y}_T) + \lambda \mathbb{E}_{\mathbf{x}_r\in\mathcal{X}_T} \mathcal{L}_{\textnormal{etx}}(\mathbf{x}_r),\\
    %      &  \textnormal{where }  \mathcal{L}_{\textnormal{etx}}(\mathbf{x}_r)=
    %     e^{\mathcal{L}_{\textnormal{tx}}(\mathbf{x}_r)}.
    % \end{array}
    % \end{equation}
    % We denote the above two methods as tx and etx, respectively.

    \textbf{R2ET-mm}$_{\backslash \mathbf{H}}$:
    Similar to \textbf{R2ET}$_{\backslash \mathbf{H}}$,
    it is a variant of \textbf{R2ET-mm} but does not optimize the Hessian-related term in Eq. (\ref{eq:defense_thick}) ($\lambda_2=0$).

\end{itemize}

\subsection{Target Models}

\subsubsection{Introduction to Siamese Network}
\label{sec:intro_to_SN}
An SN accepts a pair of samples,
$\mathbf{x}^s$ and $\mathbf{x}^t$,
as inputs and predicts the probability that two samples are from the same class.
The SN uses a deep network to embed each input, respectively,
and uses a similarity metric to measure the similarity of the two inputs.
An SN can be considered a binary classifier.
Specifically,
the prediction for class 1 (two samples from the same class),
$\Pr(y=1|\mathbf{x}^s,\mathbf{x}^t)$,
is
\begin{equation}
    \label{eq:sn_structure}
    f^{SN}_1(\mathbf{x}^s, \mathbf{x}^t; \mathbf{w}) =
    \textnormal{sim}(\textnormal{emb}(\mathbf{x}^s; \mathbf{w}_0), \textnormal{emb}(\mathbf{x}^t; \mathbf{w}_0); \mathbf{w}_1),
\end{equation}
and $f^{SN}_0=1-f^{SN}_1$ for class 0.
$\textnormal{sim}(\cdot, \cdot; \mathbf{w}_1)$ is a similarity metric,
such as the cosine similarity,
and $\textnormal{emb}(\cdot; \mathbf{w}_0)$ is an embedding network,
such as GNN.
$\mathbf{w} = \{\mathbf{w}_0, \mathbf{w}_1\}$ is the SN's parameter set.
We denote the ground truth used in SN as
$y^{st}=\mathbbm{1}[y^s=y^t]$,
where $y^s$ is the label of $\mathbf{x}^s$ \cite{ma2019deep}.
The SN is trained using a classification loss $\mathcal{L}_{cls}$,
such as the binary cross-entropy loss.
To make a prediction for a single input,
one can further train a classifier $f^{CL}$ based on the embedding networks from the SN.
For example,
$f^{CL}(\mathbf{x}) = \textnormal{cls}(\textnormal{emb}(\mathbf{x};\mathbf{w}_0^\prime); \mathbf{w}_2)$,
where $\mathbf{w}_0^\prime$ can be the same as or retrained based on $\mathbf{w}_0$ in Eq. (\ref{eq:sn_structure}), 
and $\textnormal{cls}(\cdot;\mathbf{w}_2)$ is a classifier such as a linear model with the parameter set $\mathbf{w}_2$.

\subsubsection{Structure of Target Models}
\label{sec:structure_vanilla_model}
\noindent \textbf{Vanilla models for tabular data.}
We adopt two-layer neural networks for tabular data.
The first layer maps the input space to a 32-dimension hidden space and uses LeakyReLU as the activation function.
The second layer maps the hidden space to the output space following a sigmoid function.

\noindent \textbf{Vanilla models for image data.}
\begin{figure}
    \centering
    \begin{minipage}{\textwidth}
    \includegraphics[width=.65\textwidth]{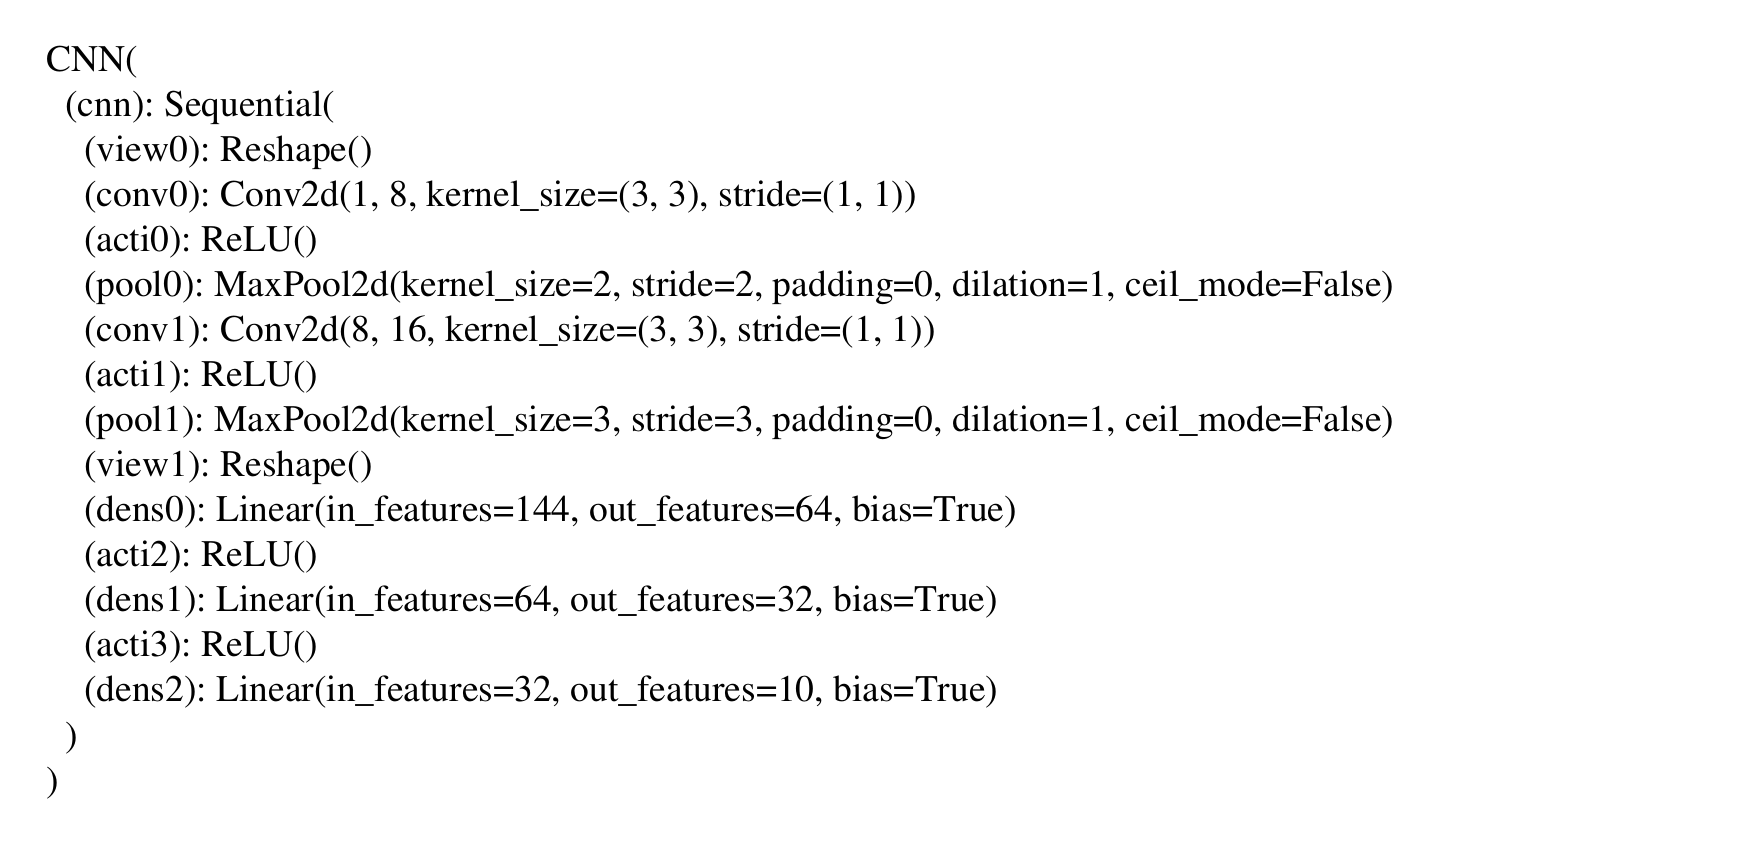}
    \end{minipage}%
    \caption{Setup of CNN for MNIST}
    \label{fig:setup_of_CNN}
\end{figure}
We use ResNet18 \cite{he2016deep} as target model on CIFAR-10.
For SN on MNIST, 
we hire a classic CNN as the embedding model,
consisting of two convolutional layers with 3*3 kernels followed by max-pooling
and three fully-connected layers;
see Fig. \ref{fig:setup_of_CNN} for details.
We use similarity metric as the cosine similarity.
The classifier is a single-layer linear model taking the outputs from the
embedding models as inputs.

\noindent \textbf{Vanilla models for graph data.}
For SN on graphs,
the embedding model is a two-layer GCN and a mean pooling is used to aggregate node features to graph-level one.
The first layer maps the input space to a 256-dimension hidden space and uses ReLU
as the activation function. The second layer maps the hidden space to a 128-dimension embedding space.
% In both cases, 
Then the cosine similarity used to
measure the similarity between two embeddings of the pair of input graphs.
The classifier is a single-layer linear model taking the outputs from the corresponding embedding models as inputs.

% \noindent \textbf{Structure of target models.}
% All methods,
% except softplus (SP),
% % and weight-decay ( WD),
% share the same structure as the Vanilla models,
% but adopt a different loss function.
% The only difference between SP and Vanilla model is the activation function,
% where SP replaces ReLU/LeakyReLU with softplus functions.
% %  WD will adopt an extra weight-decay hyperparameter during training.

\subsubsection{Methodology of Training Target Models}
\label{sec:supp_cauc}
Except CIFAR-10,
we train all the models starting from random initialization by default,
although we do provide results based on the retraining schema in \ref{sec:sensitivity_analysis_experiments},
where we retrain model based on the high-cAUC Vanilla models.
Since it takes a long time to train ResNet on CIFAR-10,
target models for CIFAR-10 are retrained from Vanilla model,
and retrained models are equipped with softplus as activation function due to the lack of softmax in ResNet.
All models are trained on the training set, 
and the ones with high cAUC for prediction and high P@$k$ for explanations on the validation set will be adopted as the outstanding models for the corresponding method.
Specifically,
% we first filter out models with low cAUC.
We choose the last model with cAUC higher than a \textit{threshold} on the validation set.
% to ensure that the model accuracy does not drop too much while making the defense strategy as effective as possible. 
The threshold depends on the Vanilla model's cAUC.
In practice, 
vanilla models achieve cAUC to 
0.87, 0.64, 0.83, 0.99, 0.87, 0.69, and 0.76 
on Adult, Bank, COMPAS, MNIST, CIFAR-10, BP, ADHD, respectively.
Correspondingly,
we set the cAUC threshold for other models as
0.86, 0.63, 0.83, 0.99, 0,86 0.67, and 0.74.
% On ADHD and BP, 
% we choose the model with the highest AUC on the validation set, 
% since the accuracy of the model is susceptible to defensive strategies.
We then select the outstanding models with the highest P@$k$ out of these high cAUC models on the validation set.
If not specified,
all results shown in tables and figures are from the test set.

\subsubsection{Saliency Maps of Target Models}
We use the absolute gradient values as the explanation for tabular datasets.
For MNIST, we use the absolute gradient values as the explanations, 
and normalize it so that the sum of all elements is one.
For CIFAR-10, the sum of the absolute gradient values are used as the explanations.
For graph data, 
we use element-wise multiplication of the gradient and the input as the explanation \cite{adebayo2018sanity}.
% As mentioned before,
Since the graphs in BP and ADHD are undirected, 
we focus on the upper triangular adjacency matrix in the explanation,
% (other elements are set to 0),
and then normalize it so that the sum of these elements is one.

\subsection{Experimental Settings and More Results}
\subsubsection{General Settings}
\label{sec:general_settings}
% Running Environment,

% Selection (range) of hyperparameters: 
% $\kappa$ in est-Hessian,
% $\rho$ in softplus,
% $ WD$ in weight-decay,
% $\lambda$ for regularization.
% And any others.

% \noindent \textbf{Optimization of ERAttack and Connection with PGD.}
\noindent \textbf{Attack targets on explanation ranking.}
% \subsection{Explanation Ranking Thickness as Attack Goal}
% \label{sec:ranking_thickness_attack}
% In the view of attackers,
The goal of attackers is to find an optimal perturbation $\delta^\ast$ on the input $\mathbf{x}$ to mess up the original feature ranking.
Intuitively, 
the attackers 
flip the relative ranking between ($i,j$) features for as many pairs as possible.
However, 
the ranking explanation thickness in Eq. (\ref{eq:topk_rank_thick}) is non-differentiable due to the indicator function and the integration over $t$.
Thus, 
we replace the indicator function with a differentiable monotonically increasing function of $h$ to measure the gaps between any two features' importance, 
e.g., $h(\mathbf{x},i,j)$ or $\exp\{h(\mathbf{x},i,j)\}$.
In this way, 
it is differentiable and can be handled by continuous numerical optimization algorithms.
% Another merit is that $h(\mathbf{x},i,j)$ is more ``precise'' 
% since it has a fine-grained sense about how large the gap between two features is.
Formally,
we consider the following Explanation Ranking Attack (ERAttack) objective:
\begin{equation}
\label{eq:attack_thick}
    \delta^\ast (\mathbf{x}) = 
    % \argmin_ {\| \delta \|_2 \leq \epsilon}
    % \int_0^1 
    % \sum_{i=1}^k \sum_{j=k+1}^n
    % h(\mathbf{x}(t), i,j) dt
    % =
    \argmin_ {\| \delta \|_2 \leq \epsilon}
    \int_0^1 
    \sum_{i=1}^k \sum_{j=k+1}^n
    h(\mathbf{x} + t \delta, i,j) dt
    , 
    % \right],
\end{equation}
where $\mathbf{x}$ is the target sample to attack,
and we denote $\mathbf{x}^\prime=\mathbf{x}+\delta$ as the adversarial sample.
We do not explicitly present constraints as Eq. (\ref{eq:attack_general}),
and deal with these constraints by constrained optimization algorithms empirically.
% More details can be found in Appendix \ref{sec:append_experiments}.

It is infeasible to optimize Eq. (\ref{eq:attack_thick}) by gradient descent directly due to the integration over $t$.
We propose finding the optimal perturbations in the PGD-style \cite{madry2017towards},
which searches the optimal adversarial sample by iteratively moving a small distance towards the goal function.
Assume that the ERAttack searches the optimal $\delta^\ast(\mathbf{x})$ starting from $\mathbf{x}^0\coloneqq\mathbf{x}$ within $T$ iterations. 
We first approximate the integration by summation,
$\frac{1}{T} \sum_{t=1}^T \sum_{i=1}^k \sum_{j=k+1}^n
h(\mathbf{x} + \frac{t}{T} \delta, i,j)$.
% Inspired by PGD \cite{madry2017towards},
% which searches the optimal adversarial sample by iteratively moving small distance towards the goal function,
Instead of directly searching the optimal $\delta^\ast$ by solving Eq. (\ref{eq:attack_thick}) for $\mathbf{x}$,
we decompose the optimization into $T$ steps.
In the $t$-th attacking iteration,
% The key idea is to 
we search for the optimal perturbation $\delta^t$ to minimize $\frac{1}{T}\sum_{i=1}^k \sum_{j=k+1}^n h(\mathbf{x}^t,i,j)$ for the intermediate point $\mathbf{x}^t \coloneqq \mathbf{x}^{t-1}+\delta^{t-1}$.
% The integration with respect to $t$ indicates that the objective function is supposed to be minimized for every intermediate small step $dt$.
Eventually, 
the ERAttack ends at an adversarial sample $\mathbf{x}^\prime=\mathbf{x}^T$ after traveling a distance of $\epsilon$ for $T$ iterations.
Note that $\mathbf{x}+\frac{t}{T}\delta$ is not necessarily equivalent to $\mathbf{x}^t$,
although they are empirically consistent.
% as shown in experiments.
% Optimizing Eq. (\ref{eq:attack_thick}) is naturally consistent with PGD \cite{madry2017towards}, 
% which searches the optimal adversarial sample by iteratively moving small distance towards the goal function.

\noindent \textbf{Hyperparamters.}
We pick $k=8$ for three tabular data,
$k=100$ for CIFAR-10,
and $k=50$ for MNIST and graphs by default.
We set the maximal training epoch as 300 for three tabular data,
100 for MNIST, 
and 10 for two graph datasets, BP and ADHD.
The maximal retraining epoch for CIFAR-10 is set as 10.
Almost all models are guaranteed to converge within given maximal epochs,
except when the regularization term weights are too large.
% For the maximum training epoch, we set 100 epochs on MNIST and 10 epochs on BP and ADHD, 
% both of which can guarantee model convergence except that the regular term weights are too large. 
The learning rate is set to 1e-2 for three tabular data, 1e-3 for MNIST, 1e-2 for CIFAR-10, and 1e-4 for BP and ADHD.
The early stop for three tabular data is 30, and no early stop is set for the image and graph datasets.
Except in the sensitivity analysis in Appendix \ref{sec:sensitivity_analysis_experiments},
we set $k^\prime=k$ for R2ET and its variants for three tabular datasets and image datasets,
% Since for R2ET-mm and R2ET-$\textnormal{mm}_{\backslash H}$, 
% setting $k^\prime=k$ reduces cAUC on BP and ADHD, 
and $k^\prime=20$ for BP and ADHD.
% for both methods on both datasets.
In each iteration,
R2ET maintains the ranking from model in the previous iteration.

As for the hyperparameters used in attacks, 
we conduct attacks in a PGD-style \cite{madry2017towards} for at most 1000 iterations for tabular datasets, 
and perturb input with a 1e-3 budget in each iteration.
Thus, 
each input in tabular datasets can be manipulated with at most $\epsilon=10^{-3}*1000=1$ budget. 
The budget is set as 100 * 5e-2 for CIFAR-10,
% For image and graph datasets, 
and 100 * 1e-2 for the rest.
% the number of iterations is 100 with 1e-2 budget. 
At each iteration,
the infinity norm of 
% the difference between the perturbed input and the original input 
the perturbations
is restricted to be no more than 5 for images and 0.2 for graphs.

% For model selection in each hyperparameter setting, 
% on MNIST, 
% we choose the highest AUC on the validation set for the basic ReLU model. 
% For other methods, 
% we choose the last model with AUC $>$ 0.99 on the validation set, 
% in order to ensure that the model accuracy does not drop too much while making the defense strategy as effective as possible. 
% On ADHD and BP, we choose the model with the highest AUC on the validation set, 
% since the accuracy of the model is susceptible to defensive strategies.

% For the hyperparameters in baselines and our proposed methods, 
% we search on the validation set and select the one with the highest P@$k$, 
% and AUC not much lower than the basic ReLU model as the final model to test on the test set. 
% More specifically, 
% the AUC of the basic ReLU model on the validation set of MNIST is greater than 0.99, 
% about 0.69 for BP, and about 0.76 for ADHD. 
% Therefore we remove those with AUC less than 0.99 on MNIST, 
% less than 0.67 on BP and less than 0.74 on ADHD. 
\noindent \textbf{Candidate range of parameters.}
% To estimate the Hessian norm by the finite differential method,
We search $\kappa$ for estimating Hessian norm by the finite differential in Est-H from $\{1e-6, 1e-5, ..., 1e-2\}$.
$\rho$ in SP from $\{0.5, 1, 5, 10, 100\}$, 
and the weight-decay parameter in WD from $\{5e-5, 5e-4, 5e-3, 1e-2, 5e-2\}$.
As for all other (single) regularization-based methods,
$\lambda$ can be drawn from $\{0.01, 0.1, 1, 5, 10, 100\}$.
As for the dual regularization methods, such as R2ET,
we adopt the following settings for the weights.
% for dual regularization methods, such as R2ET.
$\lambda_1$ and $\lambda_2$ are selected as the same as the best $\lambda$ for $\textnormal{R2ET}_{\backslash H}$ and est-H, respectively.
Alternatively,
we simply set $\lambda_1=\lambda_2=\lambda$, and $\lambda$ can be drawn from $\{0.01, 0.1, 1, 5, 10, 100\}$.
% (on graph and image datasets).

\noindent \textbf{Running environment.}
We majorly conduct experiments for three tabular data and CIFAR-10 on the following two machines.
Both come with a 16-core Intel Xeon processor and four TITAN X GPUs.
One installs 16.04.3 Ubuntu with 3.8.8 Python and 1.7.1 PyTorch,
and the other installs 18.04.6 Ubuntu with 3.7.6 Python and 1.8.1 PyTorch.
The MNIST and graph datasets are run on a machine with two 10-core Intel Xeon processors and five GeForce RTX 2080 Ti GPUs, which installs 18.04.3 Ubuntu with 3.9.5 Python and 1.9.1 PyTorch.

\subsubsection{Settings for Correlation Experiments and More Results}
\label{sec:correlation_experiment_appendix}
Sec. \ref{sec:relation_thickness_other_metric} explores the correlation between the manipulation epochs and thickness and Hessian norm,
% other metrics, 
% including thickness, P@$k$, MSE, PCC and Hessian norm,
based on R2ET results on COMPAS datasets.
Here,
we provide more results in terms of different models on various datasets.
Specifically,
as shown in Fig. \ref{fig:append_correlation_manipulation_thickness},
we consider different datasets and methods, such as Vanilla, est-H, and R2ET.
Since images and graphs have many more features than the three tabular datasets, 
almost all samples will generate swapped feature pairs under the first epoch of attack,
making the previously defined manipulation epoch metric meaningless.
% To address this issue, 
Alternatively,
we set the manipulation epoch metric for graph and image datasets to record the first epoch where P@$k$ drops below $0.8$.
We do not plot the results on Bank dataset, 
where R2ET achieves 100$\%$ P@$k$,
thus, corresponding correlations and figures are not attractive.
Fig. \ref{fig:append_correlation_manipulation_thickness} presents the correlations between manipulation epochs and the other four metrics.
Except thickness measured by adversarial samples and Hessian norm as used in Sec. \ref{sec:relation_thickness_other_metric} (shown in the first two columns),
we additionally show the thickness measured by either the average or minimal of a few Gaussian samples.
As mentioned in Sec. \ref{sec:ranking_thickness_def},
different sampling distribution over $\mathbf{x}^\prime$ is designed for distinct scenarios.
Specifically,
when samples $\mathbf{x}^\prime$ are drawn from Gaussian distribution,
the thickness is specific to the ranking robustness under \textit{random noise} \cite{zhou2006ranking}, 
instead of \textit{adversarial attacks} being evaluated by adversarial samples.
Even though the thickness evaluated by Gaussian distribution is not specific to adversarial attacks,
it is evident that the corresponding correlations are much higher than that between the manipulation epoch and Hessian norm.

\begin{figure*}
    \centering
    \begin{minipage}{.25\textwidth}
    \includegraphics[width=\textwidth]{figs/adult_Thickness and manipulation epoch_vanilla.pdf}
    % \hspace{.25cm}%
    \end{minipage}%
    \begin{minipage}{.25\textwidth}
    \includegraphics[width=\textwidth]{figs/adult_Hessians and manipulation epoch_vanilla.pdf}
    \end{minipage}%
    \begin{minipage}{.25\textwidth}
    \includegraphics[width=\textwidth]{figs/adult_Gaussian Thickness and Manipulation epoch_vanilla.pdf}
    \end{minipage}%
    \begin{minipage}{.25\textwidth}
    \includegraphics[width=\textwidth]{figs/adult_Minimal Gaussian Thickness and Manipulation epoch_vanilla.pdf}
    \end{minipage}%
    % \begin{minipage}{.25\textwidth}
    % \includegraphics[width=\textwidth]{figs/adult_lower bound and manipulation epoch_vanilla.pdf}
    % \end{minipage}
    \\
    \begin{minipage}{.25\textwidth}
    \includegraphics[width=\textwidth]{figs/adult_Thickness and manipulation epoch_est-H.pdf}
    % \hspace{.25cm}%
    \end{minipage}%
    \begin{minipage}{.25\textwidth}
    \includegraphics[width=\textwidth]{figs/adult_Hessians and manipulation epoch_est-H.pdf}
    \end{minipage}%
    \begin{minipage}{.25\textwidth}
    \includegraphics[width=\textwidth]{figs/adult_Gaussian Thickness and Manipulation epoch_est-H.pdf}
    \end{minipage}%
    \begin{minipage}{.25\textwidth}
    \includegraphics[width=\textwidth]{figs/adult_Minimal Gaussian Thickness and Manipulation epoch_est-H.pdf}
    \end{minipage}%
    % \begin{minipage}{.25\textwidth}
    % \includegraphics[width=\textwidth]{figs/adult_lower bound and manipulation epoch_est-H.pdf}
    % \end{minipage}
    \\
    \begin{minipage}{.25\textwidth}
    \includegraphics[width=\textwidth]{figs/adult_Thickness and manipulation epoch_BERD.pdf}
    % \hspace{.25cm}%
    \end{minipage}%
    \begin{minipage}{.25\textwidth}
    \includegraphics[width=\textwidth]{figs/adult_Hessians and manipulation epoch_BERD.pdf}
    \end{minipage}%
    \begin{minipage}{.25\textwidth}
    \includegraphics[width=\textwidth]{figs/adult_Gaussian Thickness and Manipulation epoch_BERD.pdf}
    \end{minipage}%
    \begin{minipage}{.25\textwidth}
    \includegraphics[width=\textwidth]{figs/adult_Minimal Gaussian Thickness and Manipulation epoch_BERD.pdf}
    \end{minipage}%
    % \begin{minipage}{.25\textwidth}
    % \includegraphics[width=\textwidth]{figs/adult_lower bound and manipulation epoch_BERD.pdf}
    % \end{minipage}
    \\
    \begin{minipage}{.25\textwidth}
    \includegraphics[width=\textwidth]{figs/compas_Thickness and Manipulation epoch.pdf}
    % \hspace{.25cm}%
    \end{minipage}%
    \begin{minipage}{.25\textwidth}
    \includegraphics[width=\textwidth]{figs/compas_Hessians and manipulation epoch.pdf}
    \end{minipage}%
    \begin{minipage}{.25\textwidth}
    \includegraphics[width=\textwidth]{figs/compas_Gaussian Thickness and Manipulation epoch.pdf}
    \end{minipage}%
    \begin{minipage}{.25\textwidth}
    \includegraphics[width=\textwidth]{figs/compas_Minimal Gaussian Thickness and Manipulation epoch.pdf}
    \end{minipage}%
    % \begin{minipage}{.25\textwidth}
    % \includegraphics[width=\textwidth]{figs/compas_lower bound and manipulation epoch.pdf}
    % \end{minipage}
    \\
    \begin{minipage}{.25\textwidth}
    \includegraphics[width=\textwidth]{figs/MNIST_Thickness and manipulation epoch.pdf}
    % \hspace{.25cm}%
    \end{minipage}%
    \begin{minipage}{.25\textwidth}
    \includegraphics[width=\textwidth]{figs/MNIST_Hessians and manipulation epoch.pdf}
    \end{minipage}%
    \begin{minipage}{.25\textwidth}
    \includegraphics[width=\textwidth]{figs/MNIST_Gaussian Thickness and manipulation epoch.pdf}
    \end{minipage}%
    \begin{minipage}{.25\textwidth}
    \includegraphics[width=\textwidth]{figs/MNIST_Minimal Gaussian Thickness and Manipulation epoch.pdf}
    \end{minipage}%
    \\
    \begin{minipage}{.25\textwidth}

    \includegraphics[width=\textwidth]{figs/ADHD_Thickness and manipulation epoch.pdf}
    % \hspace{.25cm}%
    \end{minipage}%
    \begin{minipage}{.25\textwidth}
    \includegraphics[width=\textwidth]{figs/ADHD_Hessians and manipulation epoch.pdf}
    \end{minipage}%
    \begin{minipage}{.25\textwidth}
    \includegraphics[width=\textwidth]{figs/ADHD_Gaussian Thickness and manipulation epoch.pdf}
    \end{minipage}%
    \begin{minipage}{.25\textwidth}
    \includegraphics[width=\textwidth]{figs/ADHD_Minimal Gaussian Thickness and Manipulation epoch.pdf}
    \end{minipage}%
    \\
    \begin{minipage}{.25\textwidth}
    \includegraphics[width=\textwidth]{figs/BP_Thickness and manipulation epoch.pdf}
    % \hspace{.25cm}%
    \end{minipage}%
    \begin{minipage}{.25\textwidth}
    \includegraphics[width=\textwidth]{figs/BP_Hessians and manipulation epoch.pdf}
    \end{minipage}%
    \begin{minipage}{.25\textwidth}
    \includegraphics[width=\textwidth]{figs/BP_Gaussian Thickness and manipulation epoch.pdf}
    \end{minipage}%
    \begin{minipage}{.25\textwidth}
    \includegraphics[width=\textwidth]{figs/BP_Minimal Gaussian Thickness and Manipulation epoch.pdf}
    \end{minipage}%
    
    \caption{We show the correlation between the manipulation epoch and other metrics, including thickness evaluated by adversarial samples, Hessian norm, and thickness evaluated by (mean and min of) Gaussian samples for different models in various datasets.
    From top to bottom:
    Vanilla, est-H models on Adult, respectively.
    R2ET models on Adult, COMPAS, MNIST, ADHD, and BP, respectively.
    }
    \label{fig:append_correlation_manipulation_thickness}
\end{figure*}

\subsubsection{More Results for Case Study}
\label{sec:case_study_more_results}
In Sec. \ref{sec:case_study}, 
we demonstrate the robust and plausible advantages of R2ET and R2ET-mm over Vanilla and weight decay methods through case studies. 
In Fig. \ref{fig:case_study_all}, 
we provide the results of other methods mentioned in Sec. \ref{sec:method_to_compare}, 
demonstrating the advantages of R2ET and R2ET-mm over others.

\begin{figure*}
    \centering
    \begin{minipage}{\textwidth}
    \includegraphics[width=\textwidth]{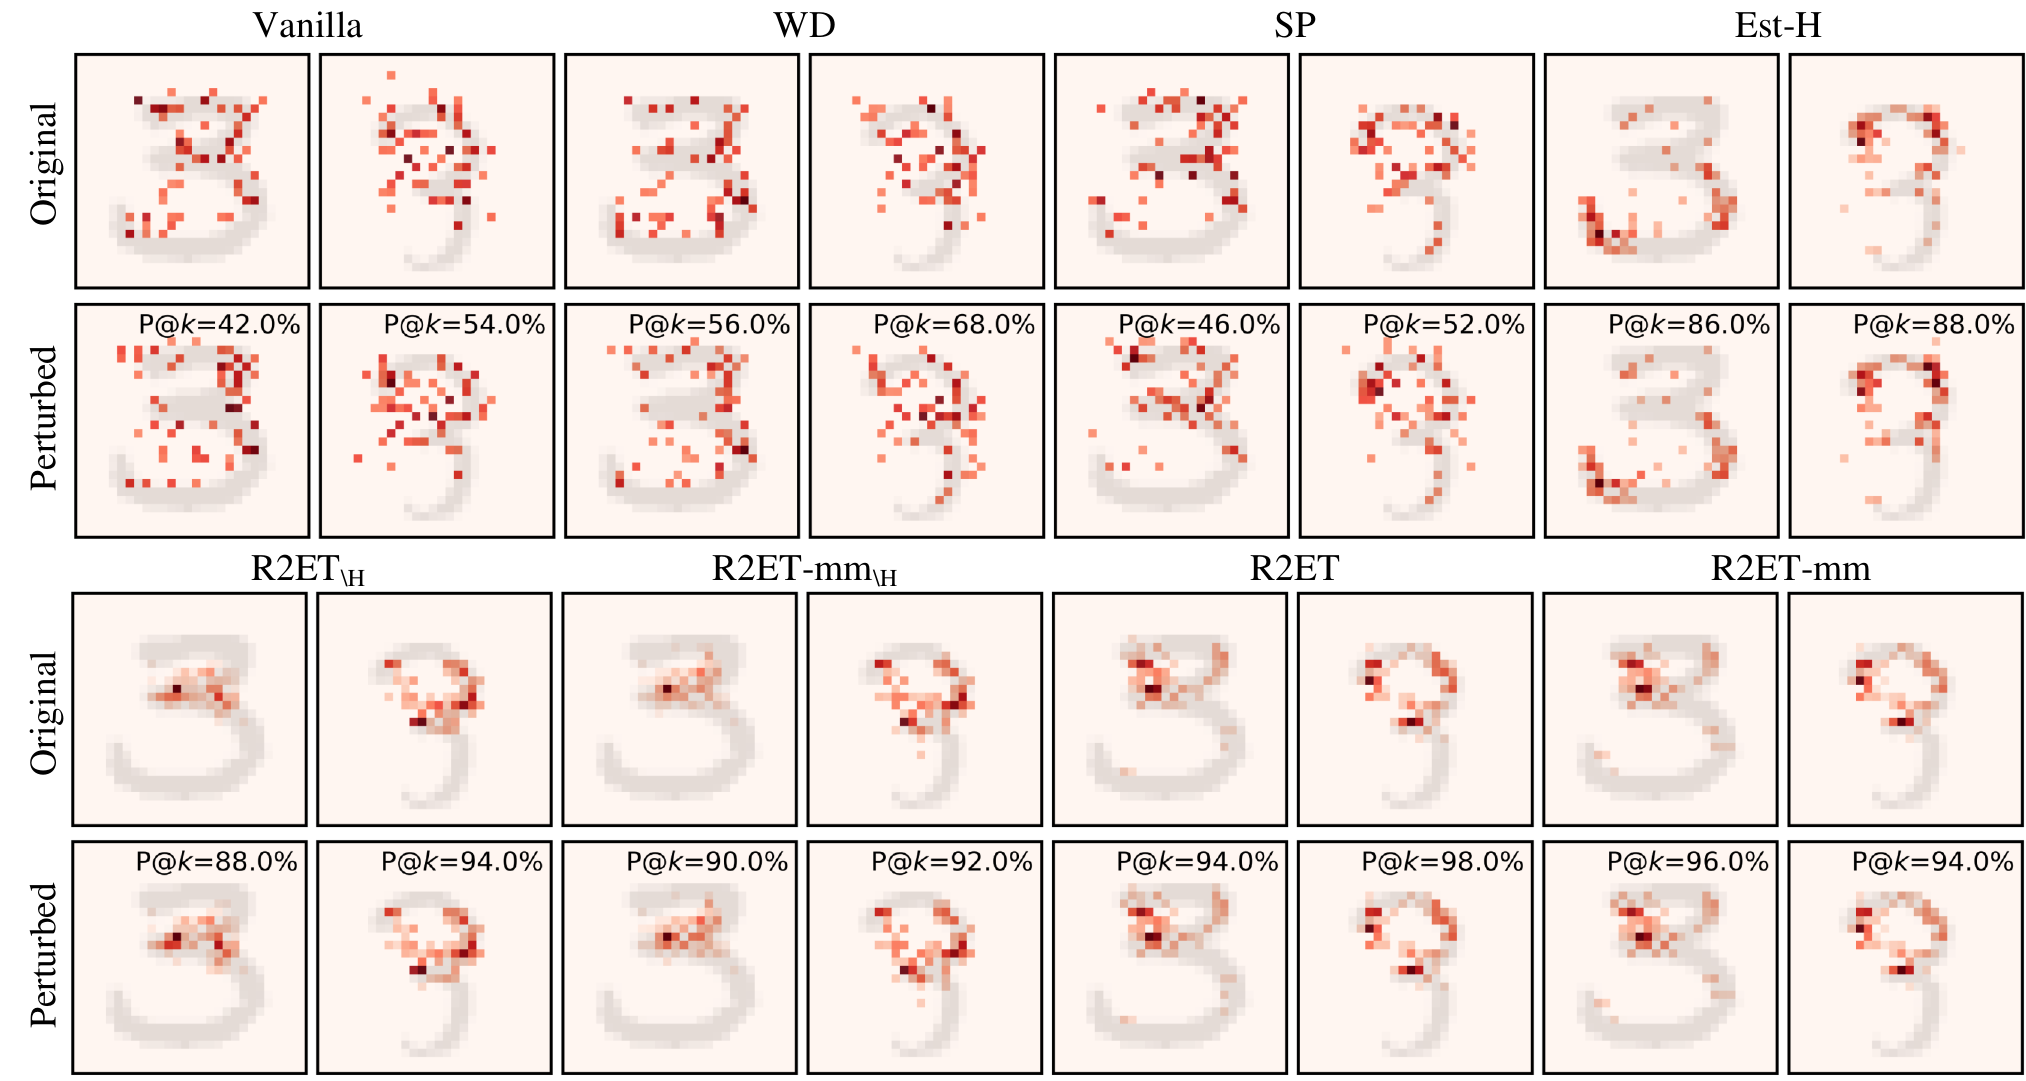}
    % \hspace{.25cm}%
    \end{minipage}%
    \\
    \begin{minipage}{\textwidth}
    \includegraphics[width=\textwidth]{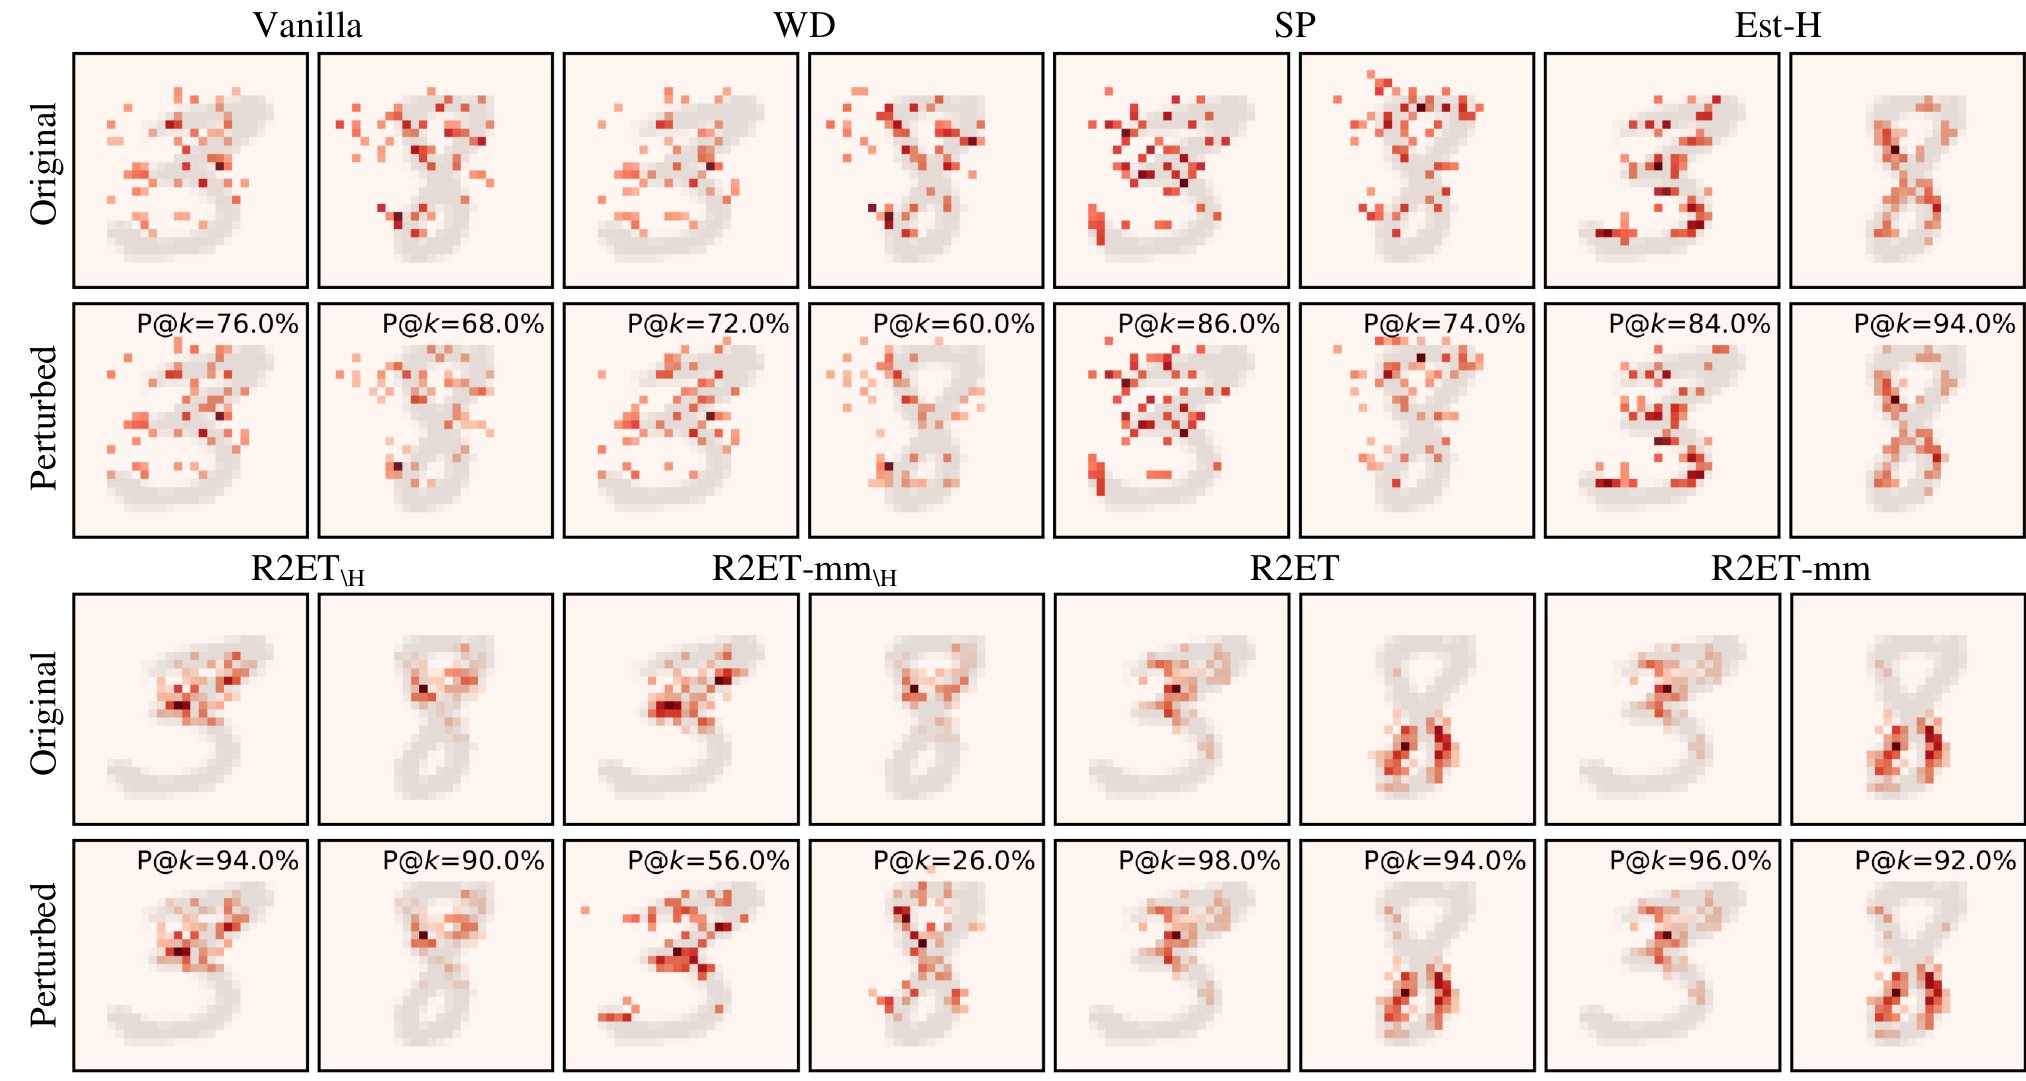}
    % \hspace{.25cm}%
    \end{minipage}%
    \caption{
    Saliency maps with respect to the original image pair and the image pair perturbed under ERAttack for all methods mentioned in Sec. \ref{sec:method_to_compare} in SNs. 
    The red pixels are the top 50 important features in saliency maps, with darker colors meaning more important. P@$k$ implies the ratio of the top 50 important features of saliency maps that overlap before and after ERAttack for the corresponding sample.
    }
    \label{fig:case_study_all}
\end{figure*}

\subsubsection{Constrained Optimization}
\label{sec:constrained_opt_appendix}
\begin{figure*}
    \centering
    \begin{minipage}{.35\textwidth}
    \includegraphics[width=\textwidth]{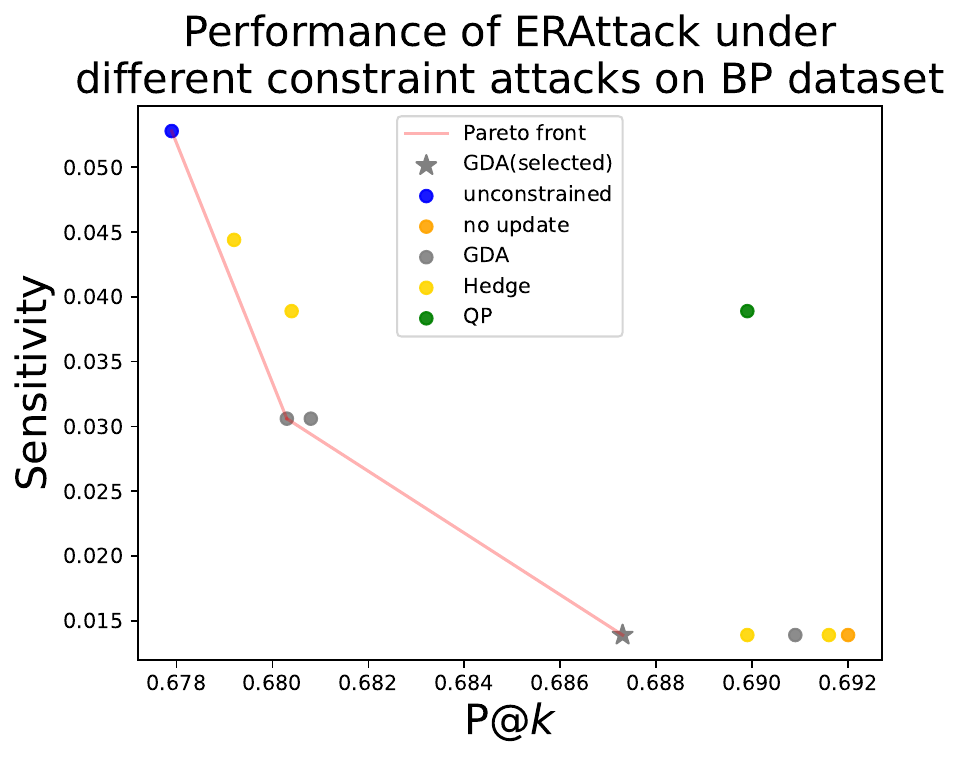}
    % \hspace{.25cm}%
    \end{minipage}%
    \begin{minipage}{.35\textwidth}
    \includegraphics[width=\textwidth]{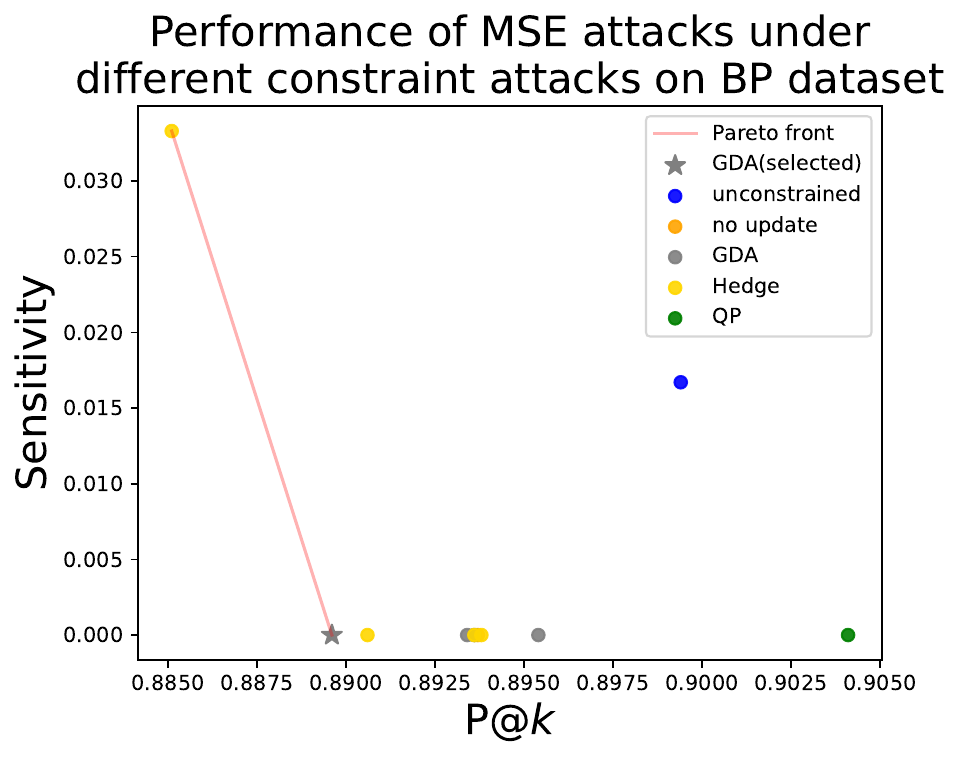}
    % \hspace{.25cm}%
    \end{minipage}%
    \\
    \begin{minipage}{.35\textwidth}
    \includegraphics[width=\textwidth]{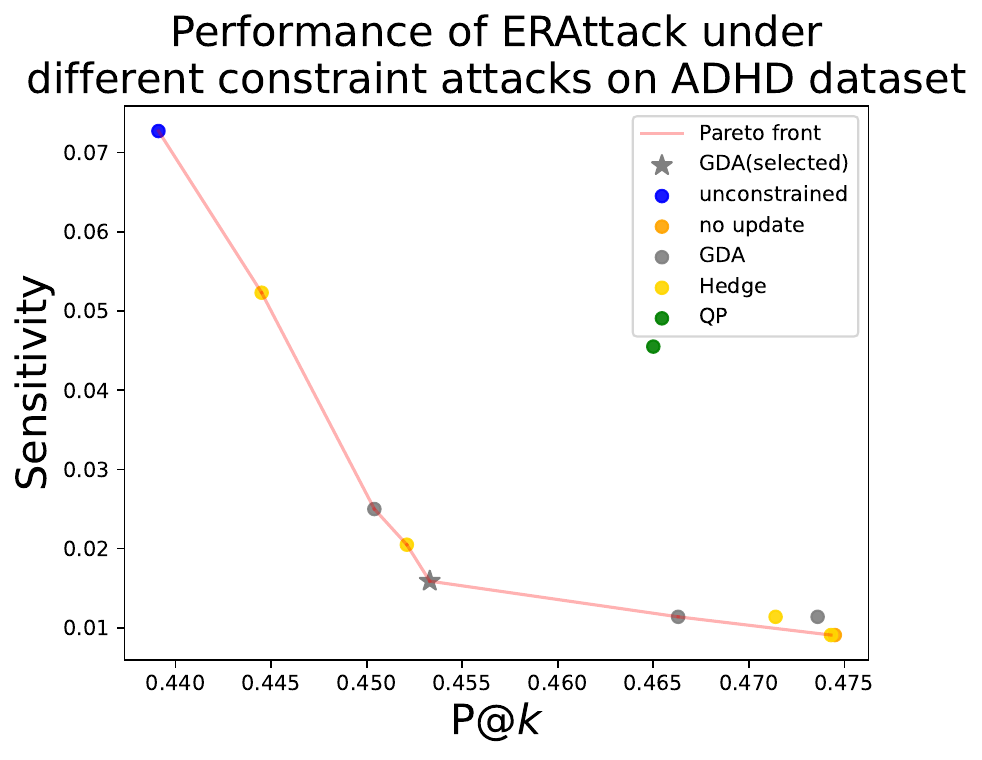}
    % \hspace{.25cm}%
    \end{minipage}%
    \begin{minipage}{.35\textwidth}
    \includegraphics[width=\textwidth]{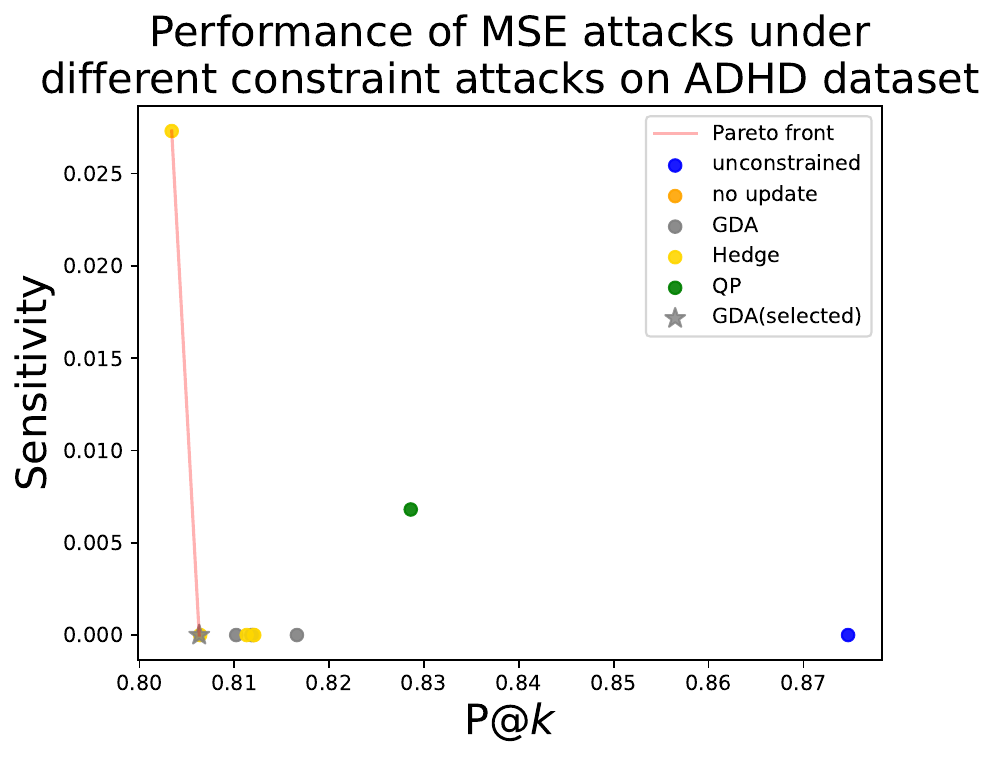}
    % \hspace{.25cm}%
    \end{minipage}%
    \caption{
    Performance of different constrained ERAttack and MSE attacks on BP and ADHD for Vanilla.
    Points in different colors represent different constraint attack methods, 
    and the same color represents the same method with a different step-size.
    The point crossed by the red line is the attack method on the Pareto front, 
    and the asterisk marks the attack method selected to evaluate the defense strategy in Table \ref{tab:comprehensive_result}.
    }
    \label{fig:attack_performance}
\end{figure*}

In Sec. \ref{sec:preliminary}, 
we briefly introduce the general form of constraints for adversarial attacks against explanations.
Since defenders can catch adversarial attacks if there are \textit{any} changes in predictions,
the attackers must keep \textit{all} predictions,
one from the SN, 
and two from the classifier with respect to the inputs,
unchanged during the attacks.
% More specifically, 
% for SN, 
% the prediction of the SN and the prediction of the classifier for a pair of inputs need to be constrained to keep the predicted class unchanged during the attack, 
We formulate it as a constrained optimization problem,
% where the goal is to manipulate the explanations such as Eq. (\ref{eq:attack_thick}),
% and the constraints come from three unchanged predictions.
% % which can be transformed into an optimization problem by using symmetric KL divergence to measure the change in predictions before and after perturbation.
Specifically,
we denote the primary objective function Eq. (\ref{eq:attack_thick}) which manipulates the explanations as $g_0$, 
and three constraints used to ensure small predictions changes as $g_1,g_2,g_3$, 
respectively.
Here,
we use symmetric KL-divergence to measure the changes in predictions before and after perturbations.
% the predicted change of SN as $g_1$, and the change of the classifier's prediction of a pair of inputs as $g_2$ and $g_3$, 
Naturally,
we construct a Lagrangian function connecting the objective function and the constraints with the non-negative Lagrange multiplier $\boldsymbol{\gamma}=[\gamma_0, \gamma_1, \gamma_2, \gamma_3] \in \mathbb{R}_+^4$,
% such as 
\begin{equation}
\label{eq:lagrange_objective}
    \mathcal{L}(\mathbf{x}, \boldsymbol{\gamma}) =
    \gamma_0 g_0 (\mathbf{x}) + 
    \sum_{k=1}^3\gamma_k g_k(\mathbf{x}).
\end{equation}

Some previous works manually set $\boldsymbol{\gamma}$ as a hyperparameter by experience \cite{dombrowski2019explanations},
which cannot capture the relatives among $g_k$.
Instead, 
we care the unsatisfied constraints with higher weights by uplifting $\gamma_k$ with larger $g_k$.
% For example,
% after training several iterations,
% uplifting some $\gamma_k$ with much larger $g_k$ should be a better strategy,
% which means we consider the unsatisfied constraints with higher weights.
% To address this issue,
Thus,
we adopt the following constrained optimization methods to update both primal variables $\mathbf{x}$ and dual variables
$\boldsymbol{\gamma}$
% =[\gamma_0, \gamma_1, \gamma_2, \gamma_3] \in \mathbb{R}_+^4$ 
% in $\mathcal{L}(\mathbf{x},\boldsymbol{\gamma})$ 
simultaneously \cite{rony2020augmented,chen2021self}:

\begin{itemize}[leftmargin=*]
\item \textbf{Gradient descent ascent (GDA)} is one of the most popular algorithms to solve the nonconvex-concave minimax problems \cite{lin2020gradient}.
% which updates 
% both primal variables $\mathbf{x}$ and dual variables
% $\boldsymbol{\gamma}$ for each iteration.
Specifically,
\begin{equation}
	\label{eq:attack_GDA}
	\begin{array}{c}
    	\mathbf{x} \leftarrow \mathbf{x} - \eta_{x} \frac{\partial \mathcal{L}}{\partial \mathbf{x}},
	    \hspace{.2in}
		\boldsymbol{\gamma} \leftarrow \boldsymbol{\gamma} + \eta_{\gamma} \frac{\partial \mathcal{L}}{\partial \boldsymbol{\gamma}},
	\end{array}
\end{equation}
where $\eta_x$ and $\eta_{\gamma}$ are the learning rates.
Notice that
$\frac{\partial \mathcal{L}(\mathbf{x}, \mathbf{\gamma})}{\partial \gamma_k} = g_k, \forall i \in \{1,2,3\}$,
and $\gamma_0$ is passively updated by the normalization $\sum_{k=0}^{3}\gamma_k=1$ 
at the end of each iteration.
% Taking the partial derivative of
% $\mathcal{L}(\mathbf{x}, \mathbf{\gamma}) =
% \gamma_0 g_0 (\mathbf{x}) + 
% \sum_{k=1}^3\gamma_k g_k(\mathbf{x})$ with respect to $\gamma_k, \forall k\in \{1,2,3\}$ is $g_k$.
% Thus, the rule for updating $\mathbf{\gamma}$ is
% In each iteration, the rule for updating is
% \begin{equation}
% 	\label{eq:attack_GDA}
% 	\begin{array}{c}
% 		\mathbf{\gamma} \leftarrow \mathbf{\gamma} + \eta_{GDA}
% 		[0, g_1, g_2, g_3]
% 	\end{array}
% \end{equation}
% where $ \eta_{GDA}\in\mathbb{R}_+$ is the learning rate. 
% and after the update, 
% $\gamma_0$ will be updated passively by the normalization $\sum_{k=0}^{3}\gamma_k=1$ 
% at the end of each update.

\item 
\textbf{Hedge} is an incarnation of Multiplicative Weights algorithm that updates $\boldsymbol{\gamma}$ by using exponential factors \cite{arora2012multiplicative}. 
In each iteration, 
we first normalize $\boldsymbol{\gamma}$ such that $ \sum_{k=0}^{3}\gamma_k=1$, 
and then update $\boldsymbol{\gamma}$ by
% and then update $ \lambda^t $. The rule for weight update is 
\begin{equation}
	\label{eq:attack_Hedge}
	\begin{array}{c}
		\boldsymbol{\gamma} \leftarrow \boldsymbol{\gamma} \odot \exp^{\eta_{Hedge}[g_0, g_1, g_2, g_3]},
	\end{array}
\end{equation}
where $ \eta_{Hedge} \in \mathbb{R}_+ $ is the learning rate,
$\odot$ is the element-wise multiplication, and $\exp$ is exponential operation. 

\item 
% As mentioned in Sec.  \ref{sec:analysis_maximizing_ranking_thickness}, 
% our third weight update algorithm is to calculate the weight $ \mathbf{\gamma} $ by
An alternative way to update weights $\boldsymbol{\gamma}$ is solving a \textbf{quadratic programming (QP)} problem
\begin{equation}
	\label{eq:attack_original_problem}
	\begin{array}{cc}
		& \max_{\boldsymbol{\gamma}} -\frac{1}{2}\|\sum_{k=0}^{3}\gamma_k \nabla g_k(\mathbf{x})\|^2, \\
		& \textnormal{s.t.} \quad 
        % \mathbf{\gamma} \in \Delta^3,
        \sum_{k=0}^{3}\gamma_k=1, \quad
        \gamma_k\geq0, \forall k\in\{0,...,3\}.
	\end{array}
\end{equation}
% where $\Delta^3$ is a probability 3-simplex such that $\sum_{k=0}^{3}\gamma_k=1$ and 
% $\gamma_k\geq0, \forall k\in\{0,...,3\}$.
\end{itemize}

% To compare with the constrained attack, 
We also consider \textbf{unconstrained} attack without any constraints,
and \textbf{no update} method that fixes the weights to $ \boldsymbol{\gamma}=[0.25, 0.25, 0.25, 0.25]$ in Eq. (\ref{eq:lagrange_objective}).

In Fig. \ref{fig:attack_performance}, 
we show different constrained attack methods in terms of P@$k$ and sensitivity through scatter plots.
For attackers, 
smaller values of both sensitivity and P@$k$ are better: 
smaller sensitivity means that the constraints are satisfied better, 
and smaller P@$k$ means that more top-$k$ important features in the explanation are distorted.
% so methods on the Pareto front are our alternative attack methods. 
From methods on the Pareto front,
we pick the one with no more than 2 $\%$ sensitivity and the smallest P@$k$.
We mark the attack methods used to evaluate the defense strategies in Table \ref{tab:comprehensive_result} with asterisks in Fig. \ref{fig:attack_performance}.
% The attack methods we finally selected to be used to evaluate the defense strategies in Table \ref{tab:comprehensive_result} need to satisfy the sensitivity of at least less than 2$\%$ and the P@$k$ as small as possible, 
% which are marked with asterisk in Fig. \ref{fig:attack_performance}.
We do not use constrained attacks on three tabular datasets and MNIST because their sensitivity is 0$\%$. 
% On MNIST, for MSE attacks we use unconstrained attacks for the same reason, but for ERAttack, 
% since the sensitivity is only 0.67$\%$ and no constrained method can make it 0$\%$, so we also use the unconstrained method. 
For datasets where constrained attacks are used (BP and ADHD), we compute the metrics in Appendix \ref{sec:append_metric} by removing the few samples caught by the defenders.
% (sensitivity $> 0\%$).

In addition to sensitivity metrics, 
we also use cAUC and aAUC to measure the performance of constrained attacks in terms of accuracy.
As shown in Table \ref{tab:cAUC_and_aAUC}, 
the difference between cAUC and aAUC for all methods is no more than 0.01,
showing the success of the selected constrained attack to retain the predictions.
% that the perturbation have little effect on the accuracy of the model.
% from the absolute value of the difference between cAUC and aAUC, 
% it can be seen that except for one method, 
% which is 0.0108, 
% the others are all less than 0.01, 
% which shows that the success of the constrained attack makes the perturbation have little effect on the accuracy of the model.

\begin{table*}[!htb]
\centering
\caption{
\textbf{cAUC/aAUC} of SNs trained by different methods under ERAttack and MSE attack on ADHD and BP.}
\begin{tabular}{ c || c c | c c}
\toprule
\textbf{Method} & ADHD(ERAttack) & BP(ERAttack) & ADHD(MSE attack) & BP(MSE attack) \\
\midrule
Vanilla & 
0.7663 / 0.7729 & 0.6812 / 0.6920 &
0.7663 / 0.7659 & 0.6744 / 0.6776

\\
WD &
0.7513 / 0.7582 & 0.6739 / 0.6726 &
0.7508 / 0.7542 & 0.6753 / 0.6722

\\
SP & 
0.7443 / 0.7358 & 0.6767 / 0.6817 &
0.7395 / 0.7375 & 0.6706 / 0.6763

\\
Est-H & 
0.7619 / 0.7643 & 0.6576 / 0.6594 &
0.7618 / 0.7633 & 0.6572 / 0.6558

\\
AT & 
0.7325 / 0.7277 & 0.6405 / 0.6347 &
0.7649 / 0.7659 & 0.6728 / 0.6773

\\
\midrule
$\textnormal{R2ET}_{\backslash H}$ & 
0.7090 / 0.7153 & 0.6697 / 0.6732 &
0.7061 \ 0.7058 & 0.6665 / 0.6700

\\
R2ET-$\textnormal{mm}_{\backslash H}$ &
0.7099 / 0.7008 & 0.6711 / 0.6720 &
0.7020 / 0.7014 & 0.6642 / 0.6654

\\
\midrule
R2ET & 
0.7169 / 0.6973 & 0.6833 / 0.6839 &
0.7049 / 0.7104 & 0.6738 / 0.6780

\\
R2ET-mm &
0.7590 / 0.7633 & 0.6892 / 0.6957 &
0.7583 / 0.7580 & 0.6841 / 0.6852

\\
\bottomrule
\end{tabular}
\label{tab:cAUC_and_aAUC}
\end{table*}

\subsubsection{Accuracy-Robustness Trade-off}
\label{sec:acc_robust_trade_off}
\begin{figure*}
    \centering
    \begin{minipage}{.33\textwidth}
    \includegraphics[width=\textwidth]{figs/MNIST_P@k_cAUC.pdf}
    % \hspace{.25cm}%
    \end{minipage}%
    \begin{minipage}{.33\textwidth}
    \includegraphics[width=\textwidth]{figs/ADHD_P@k_cAUC.pdf}
    % \hspace{.25cm}%
    \end{minipage}%
    % \\
    \begin{minipage}{.33\textwidth}
    \includegraphics[width=\textwidth]{figs/BP_P@k_cAUC.pdf}
    % \hspace{.25cm}%
    \end{minipage}%
    \\
    \begin{minipage}{.33\textwidth}
    \includegraphics[width=\textwidth]{figs/MNIST_P@k_aAUC.pdf}
    % \hspace{.25cm}%
    \end{minipage}%
    %  \\
    \begin{minipage}{.33\textwidth}
    \includegraphics[width=\textwidth]{figs/ADHD_P@k_aAUC.pdf}
    % \hspace{.25cm}%
    \end{minipage}%
    \begin{minipage}{.33\textwidth}
    \includegraphics[width=\textwidth]{figs/BP_P@k_aAUC.pdf}
    % \hspace{.25cm}%
    \end{minipage}%
    \caption{
    Trade-off between explanation robustness (P@$k$) and prediction performance (cAUC/aAUC) on MNIST, BP and ADHD. 
    The points crossed by the red lines are the methods on the Pareto front, 
    and the triangular markers present R2ET and its variants.
    }
    \label{fig:acc_robust_trade_off}
\end{figure*}

% From a defender's perspective, 
A good defensive strategy should be both robust and accurate.
Authors in \cite{tsipras2018robustness} find the trade-off between 
\textit{prediction} robustness and prediction accuracy. 
This section will explore the trade-off between the \textit{explanation} robustness and prediction performance.
% Here, we show the robustness-accuracy trade-offs of the methods mentioned in Table \ref{tab:comprehensive_result} on image and graph datasets.
Specifically, 
we study the relationship between P@$k$ and cAUC/aAUC for all methods mentioned in Table \ref{tab:comprehensive_result} on MNIST, ADHD, and BP.
% In Fig. \ref{fig:acc_robust_trade_off}, we use some scatter plots to show the relationship between P@$k$ and cAUC/aAUC, which represent ranking robustness and accuracy, respectively.
For a defender, larger values of both P@$k$ and cAUC/aAUC are better: a higher P@$k$ means a more robust model, and a higher cAUC/aAUC means a more accurate model.
In Fig. \ref{fig:acc_robust_trade_off},
the methods on the Pareto front (shown by red lines) cannot be beaten by other methods under both metrics.
% Therefore, the method on the Pareto front provides a better trade-off between robustness and accuracy than other methods.
Apparently,
at least one R2ET and its variants are on the Pareto front on all datasets,
demonstrating that R2ET and its variants are more advantageous in the trade-off between robustness and accuracy.
Furthermore, 
on MNIST, 
compared with other methods on the Pareto front,
R2ET variants on the Pareto front sacrifice less AUC (less than 2$\%$) but gain significant improvements on P@$k$ (20$\%\sim$ 40$\%$).
On BP,
Est-H improve P@$k$ by 0.01 but lost about 4$\%$ AUC.
R2ET on ADHD with both high AUC and the highest P@$k$ indicates the possibility that a model can be precise and explanation-robust at the same time.

\subsubsection{Sensitivity Analysis}
\label{sec:sensitivity_analysis_experiments}

\begin{table*}[!tb]
\centering
\caption{P@$k$ (shown in percentage) of models trained by different methods under ERAttack. 
Three numbers for each method on tabular datasets present the results when $k$ is \textbf{2}, \textbf{5}, and \textbf{8}, respectively. 
And $k$ is set to \textbf{10}, \textbf{30}, and \textbf{50} on the rest datasets, respectively.
% Three numbers for each method on image and graph datasets present the results when $k$ equals to \textbf{10}, \textbf{30}, and \textbf{50}, respectively.
Exact-H and SSR are only applicable on tabular datasets due to high time complexity.}
\begin{tabular}{ c || c c c}
\toprule
\textbf{Method} & Adult & Bank
& COMPAS \\
\midrule
Vanilla & 
79.3 / 81.9 / 87.6 & 
97.9 / 81.4 / 83.0 & 
66.1 / 78.1 / 84.2
\\
WD &
100.0 / 99.8 / 91.7 & 
97.2 / 92.5 / 82.4 & 
100.0 / 88.1 / 87.7 
\\
SP & 
100.0 / 100.0 / 97.4 & 
100.0 / 99.4 / 95.4 & 
100.0 / 100.0 / 99.5
\\
Est-H & 
100.0 / 92.9 / 87.1 & 
86.9 / 83.9 / 78.4 & 
99.9 / 83.9 / 82.6 
\\
Exact-H & 
100.0 / 92.3 / 89.6 & 
92.9 / 89.1 / 81.9 & 
79.9 / 79.3 / 77.2 
\\
SSR & 
100.0 / 92.9 / 91.2 & 
87.0 / 85.8 / 76.3 & 
87.4 / 87.1 / 82.1 
\\
% AT & 
% \\
\midrule
$\textnormal{R2ET}_{\backslash H}$ & 
100.0 / 98.5 / 97.5 & 
100.0 / 96.0 / 100.0 & 
84.0 / 98.1 / 91.9
\\
R2ET-$\textnormal{mm}_{\backslash H}$ &
100.0 / 99.8 / 93.5 & 
99.2 / 94.8 / 95.8 &
100.0 / 83.7 / 95.3 
\\
\midrule
R2ET & 
100.0 / 93.2 / 92.1 & 
100.0 / 91.8 / 80.4 & 
79.4 / 88.8 / 92.0 
\\
R2ET-mm &
100.0 / 99.7 / 87.8 &
98.6 / 92.2 / 75.1 & 
89.0 / 89.0 / 82.1 
\\
\bottomrule
\toprule
% \vspace{10pt}
\textbf{Method} & MNIST & ADHD
& BP \\
\midrule
Vanilla & 
51.6 / 56.7 / 59.4 & 
39.4 / 43.2 / 45.3  & 
63.8 / 67.3 / 68.7 
\\
WD &
51.6 / 56.6 / 59.9  & 
41.0 / 46.3 / 48.6  & 
63.6 / 68.0 / 68.8 
\\
SP & 
54.9 / 60.5 / 63.1  & 
39.4 / 42.7 / 44.7  & 
63.9 / 66.9 / 67.9 
\\
Est-H & 
80.2 / 82.9 / 84.5 & 
53.3 / 56.4 / 57.1 & 
70.8 / 74.8 / 74.3 
\\
\midrule
$\textnormal{R2ET}_{\backslash H}$ & 
77.6 / 80.7 / 82.3  & 
59.3 / 62.6 / 63.1  & 
64.5 / 69.3 / 71.4 
\\
R2ET-$\textnormal{mm}_{\backslash H}$ &
76.5 / 80.0 / 81.9 & 
57.2 / 62.3 / 64.3 &
67.6 / 71.5 / 73.1 
\\
\midrule
R2ET & 
81.4 / 84.1 / 85.3 & 
70.7 / 74.1 / 73.8 & 
66.1 / 70.5 / 72.2 

\\
R2ET-mm &
80.6 / 83.5 / 84.9 &
55.3 / 58.5 / 60.1 & 
69.4 / 74.2 / 75.1
\\
\bottomrule
\end{tabular}
\label{tab:sensitivity_analysis_k}
\end{table*}

\begin{figure*}
    \centering
    \begin{minipage}{.33\textwidth}
    \includegraphics[width=\textwidth]{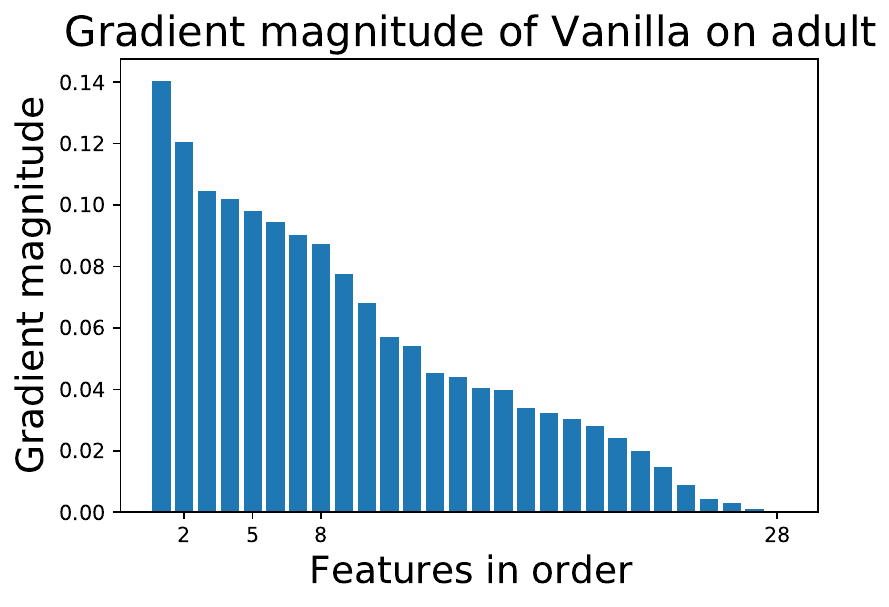}
    \end{minipage}%
    \begin{minipage}{.33\textwidth}
    \includegraphics[width=\textwidth]{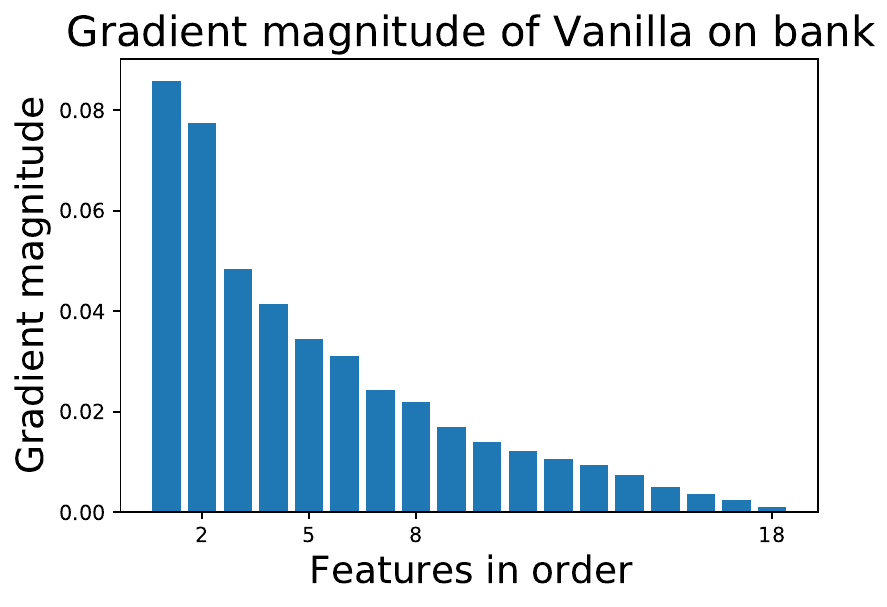}
    \end{minipage}%
    \begin{minipage}{.33\textwidth}
    \includegraphics[width=\textwidth]{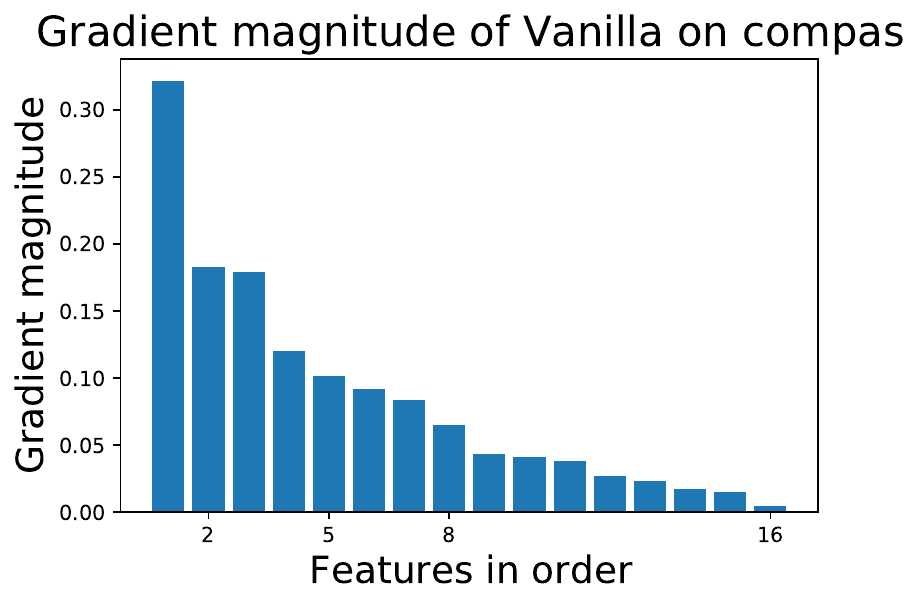}
    \end{minipage}%
    \\
    \begin{minipage}{.33\textwidth}
    \includegraphics[width=\textwidth]{figs/MNIST_Gradient magnitude of Vanilla on MNIST.pdf}
    % \hspace{.25cm}%
    \end{minipage}%
    \begin{minipage}{.33\textwidth}
    \includegraphics[width=\textwidth]{figs/ADHD_Gradient magnitude of Vanilla on ADHD.pdf}
    % \hspace{.25cm}%
    \end{minipage}%
    \begin{minipage}{.33\textwidth}
    \includegraphics[width=\textwidth]{figs/BP_Gradient magnitude of Vanilla on BP.pdf}
    % \hspace{.25cm}%
    \end{minipage}%
    \caption{
    We order the features based on the \textit{Vanilla} model's gradient magnitude with respect to each original inputs on different datasets.
    Notice that these figures would differ for various models.
    }
    \label{fig:gradient_magnitude}
\end{figure*}

In this section,
we consider the impacts of three hyperparameters or settings.

\noindent \textbf{Impacts of $\boldsymbol{k}$.}
First,
we explore whether different settings of $k$ result in similar observations and conclusions.
As shown in Table \ref{tab:sensitivity_analysis_k},
similar to the observations when $k$=8 discussed in Sec.\ref{sec:experiemnt_whole_section},
R2ET and its variants
% especially $\textnormal{R2ET}_{\backslash H}$,
stay at the top compared with other baselines for various $k$.
Besides that,
SP and est-H are very competitive and sometimes beat R2ET on tabular datasets and MNIST, respectively.
% However, 
% as shown in Table \ref{tab:comprehensive_result},
However,
they cannot perform well on other datasets.

As mentioned in Eq. (\ref{eq:upper_lower_thickness}),
the gaps of gradients of original inputs positively contribute to the thickness.
We present an auxiliary Fig. \ref{fig:gradient_magnitude},
where the features are sorted in the gradient magnitude descending orderings,
and we can easily infer the gaps between any features.
Now we focus on the trends of $k$ taking different values.
On the tabular datasets,
when $k=2$ is small, 
almost all methods have about 100$\%$ P@$k$,
indicating that even ERAttack cannot effectively manipulate the ranking in such scenarios. 
This observation occurs in most models because the top 2 features are much more significant than the rest.
In Fig. \ref{fig:gradient_magnitude},
the most important feature's magnitude is significantly larger than the rest on Bank, 
and thus Vanilla has a high P@$k$ (97.9).
However,
there is a narrow margin between the top 2 and top 3 features on COMPAS, 
and attackers can easily flip their relative rankings,
thus Vanilla's P@$k$ reduces to around 2/3.
% As a result, 
% models without boosting explanation ranking thickness also hold the top 2 features most of the time.
When $k=5$ is larger, 
P@$k$ of most non-ranking-specific methods reduce to 90$\%$ in Adult and Bank
and 80$\%$ in COMPAS.
P@$k$ further significantly reduces when $k$=8.
The key reason for the reduction is that the gaps among features on the ``long tails'' are significantly smaller than those on the top,
and usually minor perturbation is needed for a successful flip.
On MNIST, BP and ADHD,
P@$k$ for most methods increases as $k$ grows.
It seems that all methods are more efficient against ERAttack with larger $k$.
However,
the \textit{absolute number} of success manipulations for top-$k$ features increases for larger $k$.
Take Vanilla on MNIST as an example, 
ERAttack distorts the model's 5 features when $k$=10, and about 40$\%*50$=20 features when $k$=50.
Since ERAttack uses the same budget for different $k$,
it becomes harder for ERAttack to manipulate more features simultaneously (for larger $k$).
However,
it indeed kicks off more features from the top positions due to narrower margins on the long tail.
% To sum up,
% when $k=2$,
% although the Vanilla model cannot defend ERAttack,
% most existing works can save the P@$k$.
% However,
% when $k=5$,
% most existing works have relatively low P@$k$ performance.
% Their P@$k$ will further reduce when $k$=8.
% Instead,
% $\textnormal{R2ET}_{\backslash H}$ and SP always perform well for all cases.

\noindent \textbf{Impacts of the number of selected pairs.}
As discussed in Sec. \ref{sec:ranking_thickness_defense},
we can pick only $k^\prime \leq k$ number of pairs in both R2ET and $\textnormal{R2ET}$-mm methods.
For R2ET, a smaller $k^\prime \leq k$ means that 
$\sum_{i=k-k^\prime+1}^{k-1} h(\mathbf{x}, i,k) + \sum_{j=k+1}^{k+k^\prime +1} h(\mathbf{x}, k,j)$.
Here we explore the impacts of $k^\prime$ in terms of the performance of R2ET and its variants.
Notice that $\textnormal{R2ET}_{\backslash H}$ and R2ET-$\textnormal{mm}_{\backslash H}$ are the two best variants in tabular datasets.
Thus we conduct a sensitivity analysis of these two methods on Bank dataset.
We set $k=8$, 
and change $k^\prime$ from 1 to $k$.

As shown in Fig. \ref{fig:sensitivity_analysis_kprime},
both $\textnormal{R2ET}_{\backslash H}$ and R2ET-$\textnormal{mm}_{\backslash H}$ perform much better when $k^\prime > 4$ than those with $k^\prime \leq 4$.
Apparently,
when more pairs of features are taken into consideration,
R2ET and its variants have a more comprehensive view of feature rankings to maintain the rankings better.
% Besides that,
It is also worth noting that $\textnormal{R2ET}_{\backslash H}$ and R2ET-$\textnormal{mm}_{\backslash H}$ outperform almost all baselines,
except SP,
for all $k^\prime$.

\begin{figure}
    \centering
    \includegraphics[width=0.5\textwidth]{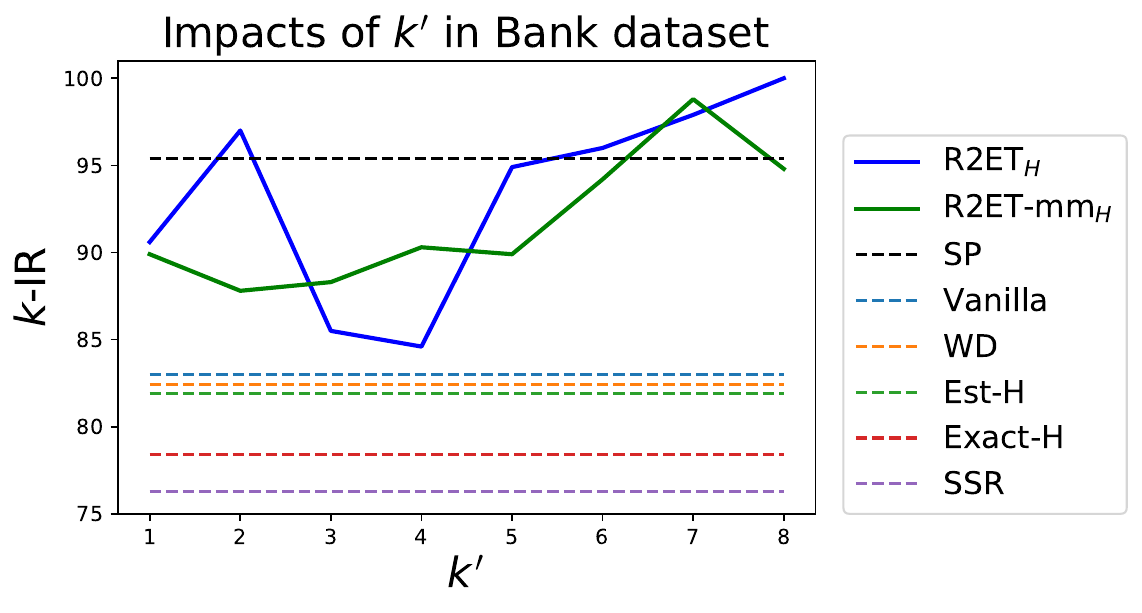}
    \caption{Sensitivity analysis on the number of selected pairs.
    $\textnormal{R2ET}_{\backslash H}$ and R2ET-$\textnormal{mm}_{\backslash H}$ are examined in Bank dataset.}
    \label{fig:sensitivity_analysis_kprime}
\end{figure}

\noindent \textbf{Impacts of pretrain / retrain.}
Lastly,
we explore how good are these methods when applying them in the retrain schema.
In previous experiments, 
all methods are trained starting from random states.
We now retrain the Vanilla models with these methods for ten epochs at most.
Since the Vanilla model has already converged and reached a good cAUC,
we assume that the Vanilla model's explanation ranking is an excellent reference,
and thus these robust methods try to maintain the Vanilla model's rankings.
Thus, we will terminate the retraining phase if
P@$k$ between Vanilla model's explanation ranking and the retrain model's ranking significantly drops,
or the retrain model's cAUC drops a lot.

Table \ref{tab:sensitivity_analysis_pretrain} present the results for comparing two training schemas.
Since the baseline SP changes the models' structure (activation function),
we do not consider it here.
Instead, 
we add one more baseline, 
CL \cite{hein2017formal},
because retraining demands much fewer training epochs, 
thus its time complexity is acceptable.
More details for CL can be found in Sec. \ref{sec:ranking_thickness_defense}.
Besides that,
\textit{none} of retrain models by Exact-H and SSR can maintain Vanilla model's explanation rankings and cAUC at the same time in Bank dataset,
and thus both are not applicable.

\subsection{SG and IG as explanation methods}
\label{sec:append_sg_ig}
Instead of using the Simple Gradient of the models with respect to inputs as the explanations, 
we here adopt two other gradient-based explanation methods, 
including SmoothGrad (SG) \cite{smilkov2017smoothgrad} and Integrated Gradients (IG) \cite{sundararajan2017axiomatic}.

SG takes random samples in a small neighborhood of input $\mathbf{x}$,
and calculates the average of the saliency maps for these neighboring samples as the final saliency map for $\mathbf{x}$. 
Particularly,
we consider adding a Gaussian noise obeying $\mathcal{N}(0, \sigma^2I)$ to the original inputs, 
\begin{equation*}
    \mathcal{I}_{SG}(\mathbf{x}) = \frac{1}{M}\sum \mathcal{I}(\mathbf{x}+\delta), 
    \quad \textnormal{s.t.} \quad
    \delta \sim \mathcal{N}(0,\sigma^2I).
\end{equation*}
$M$ is the number of neighboring samples.
% around $\mathbf{x}$.
In practice, 
we set $M$=50 for all datasets, 
and $\sigma^2=0.5, 25.5^2 \textnormal{ and } 0.01$ for tabular, image and graph datasets, respectively.

IG is defined as the integration of the saliency maps along a path from a reference point $\mathbf{x}^0$ to input $\mathbf{x}$.
Formally,
\begin{equation*}
    \mathcal{I}_{IG}(\mathbf{x}) = 
    (\mathbf{x}-\mathbf{x}^0)\int_{\alpha=0}^1 
    \frac{\partial f(\mathbf{x}^0+\alpha (\mathbf{x}-\mathbf{x}^0))}{\partial \mathbf{x}} d\alpha.
\end{equation*}
In practice, we set the reference point $\mathbf{x}^0$ as the all-zero vector, 
and approximate the integration by interpolating 100 samples between $\mathbf{x}^0$ and $\mathbf{x}$.

\noindent \textbf{Experimental results.}
Table \ref{tab:SG_IG} report P@$k$ values under ERAttack when adopting Simple Gradient, SG and IG as explanation methods, respectively.
Overall, SG and IG generate more robust explanations for most of models under attacks.
Moreover, 
the relative performance rankings among different training methods remain the same, 
no matter Simple Gradient, SG or IG is adopted as the explanation methods.
Especially,
R2ET and its variants achieve the best performance in most datasets and are compatible with other gradient-based explanation methods, such as SG and IG, for even better robustness.

Since R2ET and other baselines are \textit{training} methods,
we do NOT encourage comparing R2ET with SG, 
since SG is an \textit{explanation} method.
Both training method and explanation method change if comparing (Vanilla + SG) with (R2ET + Simple Gradient).
Instead, we compare (Vanilla + Simple Gradient) with (R2ET + Simple Gradient) to investigate the superiority of training methods, 
or to compare (R2ET + IG) with (R2ET + SG) to explore the stability of the explanation methods.

\begin{table*}[h]
\caption{P@$k$ (shown in percentage) of different models under ERAttack, $k=8$ for the first three dataset and $k=50$ for the rest.
We report P@$k$ for \textbf{Simple Gradient} (from Table \ref{tab:comprehensive_result})/\textbf{SG}/\textbf{IG} for each method-dataset combination.
}
\centering
\begin{tabular}{ c || c c c}
\toprule
\textbf{Method} & Adult & Bank
& COMPAS \\
% & MNIST & ADHD & BP \\
\midrule
Vanilla & 
87.6 / 94.0 / \textbf{71.8} & 83.0 / 90.0 / 88.1 & 84.2 / 92.9 / 94.7 
% & 59.0 / 67.9 / 82.8 & 45.5 /  & 69.4 / 
\\
WD &
91.7 / 97.3 / 55.5 & 82.4 / 91.3 / 85.7 & 87.7 / 97.4 / 99.1 
% &
% 59.1 / 68.3 / 83.0 & 47.6 / & 69.4 / 
\\
SP & 
\underline{97.4} / 95.3 / \underline{63.9} & 95.4 / 96.7 / \underline{99.9} & \textbf{99.5} / \textbf{100.0} / \textbf{100.0} 
% &
% 62.9 / 69.0 / 85.4 & 42.5 /  & 68.7 / 
\\
Est-H & 
87.1 / 93.1 / 61.5 & 78.4 / 87.3 / 82.4 & 82.6 / 89.9 / 89.9 
% &
% 85.2 / 87.9 / 89.5 & 58.2 / & \textbf{75.0} /
\\
Exact-H & 
89.6 / 95.8 / 62.1 & 81.9 / 89.7 / 90.0 & 77.2 / 91.6 / 90.8 
% &
% - / - / - & - / - / - & - / - / -
\\
SSR & 
91.2 / 93.0 / 62.5 & 76.3 / 84.9 / 85.4 & 82.1 / 96.2 / \underline{99.5} 
% &
% - / - / - & - / - / - & - / - / -
\\
AT & 68.4 / 76.6 / 60.0 & 80.0 / 85.9 / 82.6 & 84.2 / 85.9 / 82.4 
% & 56.0 / 61.5 / 79.3
\\
\midrule
$\textnormal{R2ET}_{\backslash H}$ & 
\textbf{97.5} / 97.5 / 57.3 & \textbf{100.0} / \textbf{100.0} / \textbf{100.0} & 91.0 / 96.6 / 93.6 
% &
% 82.8 / 87.1 / 89.0 & 60.7 / & 70.9 / 
\\
R2ET-$\textnormal{mm}_{\backslash H}$ &
93.5 / 97.4 / 55.9 & \underline{95.8} / \underline{97.0} / 96.3 & \underline{95.3} / 99.1 / 95.5 
% &
% 81.6 / 86.8 / 88.7 & \underline{64.2} /  & 72.4 / 
\\
\midrule
R2ET & 
92.1 / \textbf{99.3} / 54.0 & 80.4 / 88.9 / 84.4 & 92.0 / \underline{99.7} / \textbf{100.0} 
% &
% \textbf{85.7} /  & \textbf{73.8} /  & 71.5 / 
\\
R2ET-mm &
87.8 / \underline{98.6} / 54.2 & 75.1 / 85.1 / 80.3 & 82.1 / 93.5 / \underline{99.5} 
% &
% \underline{85.3} / 88.3 / 90.1 & 60.1 /  & \underline{73.8} / 
\\
\bottomrule
\end{tabular}
\begin{tabular}{ c || c | c c}
\toprule
\textbf{Method} & MNIST & ADHD & BP \\
\midrule
Vanilla & 
59.0 / 67.9 / 82.8 
& 45.5 / 39.0 / 56.9 
& 69.4 / 59.6 / 60.8
\\
WD &
59.1 / 68.3 / 83.0 
& 47.6 / 42.3 / 57.2
& 69.4 / 61.8 / 63.9
\\
SP & 
62.9 / 69.0 / 85.4 
& 42.5 / 36.9 / 54.9 
& 68.7 / 58.6 / 60.5
\\
Est-H & 
85.2 / 87.9 / 89.5 
& 58.2 / 48.9 / 54.7
& \textbf{75.0} / 63.0 / 58.5
\\
Exact-H & 
- / - / - & - / - / - & - / - / -
\\
SSR & 
- / - / - & - / - / - & - / - / -
\\
AT & 
56.0 / 61.5 / 79.3
& 59.4 / 41.2 / 43.0
& 72.0 / 56.7 / 54.4
\\
\midrule
$\textnormal{R2ET}_{\backslash H}$ & 
82.8 / 87.1 / 89.0 
& 60.7 / 56.9 / \underline{61.9}
& 70.9 / 64.2 / \textbf{66.0}
\\
R2ET-$\textnormal{mm}_{\backslash H}$ &
81.6 / 86.8 / 88.7 
& \underline{64.2} / \underline{59.5} / \underline{61.9}
& 72.4 / \underline{65.5} / 64.1
\\
\midrule
R2ET & 
\textbf{85.7} / \textbf{88.5} / \textbf{90.4} 
& \textbf{71.6} / \textbf{67.2} / \textbf{65.8}
& 71.5 / 64.0 / \underline{65.0}
\\
R2ET-mm &
\underline{85.3} / \underline{88.3} / \underline{90.1} 
& 58.8 / 50.1 / 51.4
& \underline{73.8} / \textbf{65.6} / 63.9
\\
\bottomrule
\end{tabular}
\label{tab:SG_IG}
\end{table*}

\subsection{Faithfulness of explanations on different models}
\label{sec:supp_experiment_faithfulness}

We report the faithfulness of explanations evaluated by three widely used metrics, DFFOT, COMP and SUFF, in Table \ref{tab:faithfulness}.
